# Supplementary material for: Robust Data-Driven Moving Horizon Estimation for Linear Discrete-Time Systems
Source: arXiv:2210.09017 source file (2024-02-28)
Supplement: Supplementary file 1 [file Supplementary_Material.pdf]

# Robust Data-Driven Moving Horizon Estimation for Linear Discrete-Time Systems

Tobias M. Wolff, Victor G. Lopez, *Member, IEEE*, and Matthias A. Müller, *Senior Member, IEEE*

## Abstract

In this paper, a robust data-driven moving horizon estimation (MHE) scheme for linear time-invariant discrete-time systems is introduced. The scheme solely relies on offline collected data without employing any system identification step. First, robust global exponential stability is proven under standard assumptions for a nominal case where the offline collected data are noise-free but the online measured outputs are corrupted by some non-vanishing measurement noise. Second, practical robust exponential stability is shown for the case where, in addition to the measurement noise in the online phase, the offline collected data are corrupted by some non-vanishing and bounded noise. The behavior of the novel robust data-driven MHE scheme is illustrated by means of a simulation example and compared to a standard model-based MHE, where the model is identified using the same offline data as for the data-driven MHE.

## Index Terms

data-driven state estimation, moving horizon estimation, observers for linear systems, state estimation

## I. INTRODUCTION

STATE estimation is crucial for many applications such as control, monitoring, and fault diagnosis. For linear systems, the Kalman filter [1] and the Luenberger observer [2] are the most commonly applied state estimation methods. An alternative is moving horizon estimation (MHE) [3]–[7], where the state estimation problem is centered around an optimization problem. Loosely speaking, at each time step, an optimization problem is solved to determine a state sequence that satisfies the mathematical model of the system dynamics, some known state constraints and/or disturbance bounds, and that is optimal with respect to a cost function considering the past output measurements that are inside a moving time window. Hence, the standard MHE (as well as the Kalman filter and the Luenberger observer) requires knowledge of a mathematical model describing the underlying system dynamics.

A framework for an alternative system representation that does not require any system identification was established in [8]. The main result of that work states that any system trajectory of length  $L$  of a linear time-invariant discrete-time (LTI-DT) system can be represented by using the span of a single persistently exciting trajectory measured from that system. This result, also known as Willems' fundamental lemma, has been used for data-driven simulation and control [9], for the design of data-driven linear quadratic regulators [10], and, among many other applications and extensions, for the design of model predictive controllers (MPC) [11] (with robustness guarantees [12]) purely based on input/output and possibly state data of the system. Note that all of these controller design methods do not employ any system identification step. Further work is summarized in the recent survey concerning data-driven system analysis and control in [13]. All of these aforementioned results are for discrete-time systems. Recently, a continuous-time version of the fundamental lemma has been proposed in [14].

With respect to the dual problem of data-driven state estimation, there are only few results available. One focus in this area is the design of data-driven unknown-input observers [15], [16]. A data-driven state estimation method that exploits the duality principle of control and estimation is proposed in [17]. An approach on how to perform data-driven set-based state estimation (without explicitly employing the fundamental lemma) is presented in [18].

One important difficulty in the context of data-driven state estimation, that is well known from subspace identification, is that a state sequence can only be determined up to an unknown similarity transformation when only input/output data are available [19]. This is problematic, for example, in applications where physically meaningful states are required. To overcome this issue, many of the data-driven state estimation methods require an offline (noise-free) measured state sequence [15], [17]. This form of additional knowledge will also be exploited in this work.

The contributions of this paper are the following. First, we propose a data-driven MHE framework and prove robust global exponential stability (RGES) of the resulting estimator for the case of noise-free *offline* collected input, output, and state measurements, where the *online* output measurements are corrupted by some non-vanishing measurement noise (regarded here

This project has received funding from the European Research Council (ERC) under the European Union's Horizon 2020 research and innovation programme (grant agreement No 948679).

Tobias M. Wolff, Victor G. Lopez, and Matthias M. Müller are with the Leibniz University Hannover, Institute of Automatic Control, 30167 Hannover, Germany (email: {wolff,lopez,mueller}@irt.uni-hannover.de)

as the “nominal” case<sup>1</sup>). Second, we introduce a robust data-driven MHE framework and prove practical robust exponential stability (pRES) for the case where, in addition to the measurement noise affecting the online output measurements, the offline measured state and output sequences are also subject to some bounded, non-vanishing measurement noise. This is regarded as the “robust” case. Although both proposed MHE frameworks are robust with respect to online measurement noise, the second is also robust against offline measurement noise.

Note that a preliminary version of parts of this work is available in the conference proceedings [20]. Here, we consider a different proof technique regarding the nominal case that leads to improved state estimation error bounds. Furthermore, we treat the robust case which has not been considered in [20]. Finally, our numerical example is substantially more exhaustive, since, e.g., we here compare the performance of the data-driven MHE to the performance of a model-based MHE.

The outline of this paper is the following. In Section II, we present the setup of this paper and some technical definitions. In Section III, we prove robust global exponential stability of the data-driven MHE considering noise-free offline data and noisy online output measurements. We relax the setup by allowing for noisy offline measured states and outputs and prove pRES in Section IV. We close this paper by means of an illustrative example and a conclusion in Sections V and VI, respectively.

## II. PRELIMINARIES & SETUP

The set of integers in the interval  $[a, b] \subset \mathbb{R}$  is denoted by  $\mathbb{I}_{[a,b]}$  and the set of integers greater than or equal to  $a$  by  $\mathbb{I}_{\geq a}$ . For a vector  $x = [x_1 \dots x_n]^\top \in \mathbb{R}^n$  and a symmetric positive definite matrix  $P$ , we write  $|x|_P = \sqrt{x^\top P x}$ . The minimal eigenvalue of  $P$  is denoted by  $\lambda_{\min}(P)$ . The identity matrix of dimension  $n$  is denoted by  $I_n$ . The Euclidean norm  $\|x\|_2$  is written as  $|x|$  and the infinity norm  $\|x\|_\infty$  as  $|x|_\infty$ . A stacked window of a sequence  $\{x(k)\}_{k=0}^{N-1}$  is written as  $x_{[0,N-1]} = [x(0)^\top \dots x(N-1)^\top]^\top$ . A function  $\gamma: \mathbb{R}_{\geq 0} \rightarrow \mathbb{R}_{\geq 0}$  is of class  $\mathcal{K}$ , if  $\gamma$  is continuous, strictly increasing, and  $\gamma(0) = 0$ . Furthermore, the Hankel matrix of depth  $L$  of a stacked window  $x_{[0,N-1]}$  is defined by

$$H_L(x_{[0,N-1]}) = \begin{pmatrix} x(0) & x(1) & \dots & x(N-L) \\ x(1) & x(2) & \dots & x(N-L+1) \\ \vdots & \vdots & \ddots & \vdots \\ x(L-1) & x(L) & \dots & x(N-1) \end{pmatrix}.$$

All of our results are crucially based on Willems’ fundamental lemma [8]. It holds for LTI-DT systems of the form

$$x(t+1) = Ax(t) + Bu(t) \quad (1a)$$

$$y(t) = Cx(t) + Du(t), \quad (1b)$$

where  $u(t) \in \mathbb{R}^m$ ,  $x(t) \in \mathbb{R}^n$ , and  $y(t) \in \mathbb{R}^p$ . The fundamental lemma exploits the notion of persistency of excitation.

**Definition 1:** An input sequence  $\{u(k)\}_{k=0}^{N-1}$  is persistently exciting of order  $L$  if  $\text{rank}(H_L(u_{[0,N-1]})) = mL$ .

Besides the fundamental lemma, the authors in [8] prove the following lemma.

**Lemma 1:** Suppose  $\{x(k)\}_{k=0}^{N-1}$ ,  $\{u(k)\}_{k=0}^{N-1}$  is an input/state trajectory of the controllable LTI system (1) where  $\{u(k)\}_{k=0}^{N-1}$  is persistently exciting of order  $L+n$ , then the matrix

$$\begin{bmatrix} H_1(x_{[0,N-L]}) \\ H_L(u_{[0,N-1]}) \end{bmatrix} \quad (2)$$

has full row rank.

The fundamental lemma can be formulated in the classical state space framework as follows [21], [22].

**Theorem 1:** ([21]) Suppose  $\{u(k)\}_{k=0}^{N-1}$ ,  $\{y(k)\}_{k=0}^{N-1}$  is an input/output trajectory of a controllable LTI system (1), where  $\{u(k)\}_{k=0}^{N-1}$  is persistently exciting of order  $L+n$ . Then,  $\{\bar{u}(k)\}_{k=0}^{L-1}$ ,  $\{\bar{y}(k)\}_{k=0}^{L-1}$  is a trajectory of system (1) if and only if there exists  $\alpha \in \mathbb{R}^{N-L+1}$  such that

$$\begin{bmatrix} H_L(u_{[0,N-1]}) \\ H_L(y_{[0,N-1]}) \end{bmatrix} \alpha = \begin{bmatrix} \bar{u}_{[0,L-1]} \\ \bar{y}_{[0,L-1]} \end{bmatrix}. \quad (3)$$

This important result states that any length  $L$  system trajectory of a linear controllable LTI system can be expressed in terms of a single persistently exciting system trajectory. This implies that one does not necessarily need a mathematical model of the treated system to represent system trajectories. Particularly relevant in the context of state estimation is the result summarized in the following remark.

**Remark 1:** In addition to (3), it holds that [21, Eq. (5)]

$$\bar{x}_{[0,L-1]} = H_L(x_{[0,N-1]})\alpha, \quad (4)$$

where  $\bar{x}_{[0,L-1]}$  is the state trajectory of system (1) corresponding to  $\bar{u}_{[0,L-1]}$ ,  $\bar{y}_{[0,L-1]}$  of (3) and  $x_{[0,N-1]}$  the state trajectory corresponding to  $u_{[0,N-1]}$ ,  $y_{[0,N-1]}$ .

<sup>1</sup>Strictly speaking, this case is not completely nominal, since we consider noise in the online phase. The word nominal refers here to the data in the offline phase, when the data are considered to be noise-free.

Throughout this paper, we consider an offline phase and an online phase. In the offline phase, we collect input, output and state trajectories of the considered system so that an implicit system representation according to the fundamental lemma can be established. In Section III, we assume that the offline input, output, and state measurements are noise-free. In contrast, in Section IV, we relax the setting by allowing the offline output and state measurements to be corrupted by some bounded noise. In the online phase, the states are no longer measurable and need to be estimated from input and output measurements, where the outputs are corrupted by some non-vanishing measurement noise  $v$ . Therefore, the system dynamics considered in the online phase are

$$x(t+1) = Ax(t) + Bu(t) \quad (5a)$$

$$\tilde{y}(t) = Cx(t) + Du(t) + v(t) \quad (5b)$$

that differs from (1) by the non-vanishing measurement noise  $v(t) \in \mathbb{V} \subset \mathbb{R}^p$ . We employ the notation  $y$  instead of  $\tilde{y}$  whenever  $v = 0$ .

The assumption that (potentially noisy) state measurements are available in an offline phase could be restrictive in general. However, it is satisfied in a broad range of applications where the states are measurable using, e.g., a dedicated laboratory and specific hardware, which is not available in online operations of the system (compare also the discussion in, e.g., [15]). This assumption is indispensable for the results of our work. Loosely speaking, the online input and output measurements are combined with the offline collected input and output measurements to compute a vector  $\alpha$ . This  $\alpha$ , together with the offline collected state trajectory, generates the estimated state trajectory. This estimated state trajectory is in the same (unknown) realization (1) as the offline collected state trajectory, compare Remark 1. Note that without such an offline collected state trajectory, the (online) state trajectory could not be correctly estimated since the realization  $(A, B, C, D)$  of system (1) is unknown (and hence different state trajectories can explain the given input/output data), as is, e.g., well known from the context of subspace identification [19].

### III. RGES OF THE DATA-DRIVEN MHE

In this section, we introduce the data-driven MHE scheme for the case where the offline collected states and outputs are noise-free. Given an estimation horizon  $L$  in  $\mathbb{I}_{>0}$ , at each time  $t \geq L$ , solve

$$\underset{\substack{\bar{x}_{[-L,0]}(t), \alpha(t), \\ \sigma_{[-L,-1]}^y(t)}}{\text{minimize}} \quad J(\bar{x}(t-L|t), \sigma_{[-L,-1]}^y(t)) \quad (6a)$$

$$\text{s. t.} \quad \begin{bmatrix} H_L(u_{[0,N-2]}^d) \\ H_L(y_{[0,N-2]}^d) \\ H_{L+1}(x_{[0,N-1]}^d) \end{bmatrix} \alpha(t) = \begin{bmatrix} u_{[t-L,t-1]} \\ \tilde{y}_{[t-L,t-1]} - \sigma_{[-L,-1]}^y(t) \\ \bar{x}_{[-L,0]}(t) \end{bmatrix} \quad (6b)$$

$$\bar{x}_{[-L,0]}(t) \in \mathbb{X} \quad (6c)$$

where

$$\begin{aligned} J(\bar{x}(t-L|t), \sigma_{[-L,-1]}^y(t)) \\ := \Gamma(\bar{x}(t-L|t)) + \sum_{k=1}^L \ell_k(\sigma^y(t-k|t)). \end{aligned} \quad (6d)$$

We denote the online measured inputs and outputs from time  $t-L$  up to time  $t-1$  by  $u_{[t-L,t-1]}$  and  $\tilde{y}_{[t-L,t-1]}$ , respectively. The estimated state sequence from time  $t-L$  up to time  $t$ , estimated at time  $t$ , is denoted by  $\bar{x}_{[-L,0]}(t) := [\bar{x}(t-L|t)^\top, \dots, \bar{x}(t|t)^\top]^\top$ . Similarly, the estimated fitting error from time  $t-L$  up to time  $t-1$ , estimated at time  $t$ , is written as  $\sigma_{[-L,-1]}^y(t)$ . Note that the estimated states  $\bar{x}_{[-L,0]}(t)$  and the estimated measurement noise  $\sigma_{[-L,-1]}^y(t)$  (together with  $\alpha(t)$ ) are decision variables of problem (6). The left-hand side of (6b) contains the Hankel matrices (of depth  $L$  or  $L+1$ ) of the offline collected inputs, outputs, and states. The superscript  $d$  stands for offline collected data. The optimizers of problem (6) are denoted by  $\hat{x}_{[-L,0]}(t)$ ,  $\hat{\sigma}_{[-L,-1]}^y(t)$ , and  $\hat{\alpha}(t)$ . Finally, we define the state estimate at time  $t$  by  $\hat{x}(t) := \hat{x}(t|t)$ , corresponding to the last element of the optimal sequence  $\hat{x}_{[-L,0]}(t)$ . As usual in MHE [23], [24], we can incorporate knowledge about the estimated state sequence in form of state constraints, compare (6c). These constraints are usually inherently satisfied by the system states such as, e.g., nonnegativity constraints of concentrations in a chemical reactor or serum hormone concentrations.

We introduce the fitting error  $\sigma_{[-L,-1]}^y(t)$  in the optimization problem since the noisy online output measurements  $\tilde{y}$  might not be in the span of the noise-free, offline collected outputs  $y^d$  (similar to data-driven MPC, where the future predicted outputs might not be in the span of the offline collected data [11], [12]). This fitting error is incorporated in the cost function (6d), so that the difference between the online measured outputs and the reconstructed outputs remains small. The stage costs  $\ell_k$  are defined as

$$\ell_k(\sigma^y(t-k|t)) := |\sigma^y(t-k|t)|_R^2 \rho^k \quad (7)$$

for a weighting matrix  $R$  and a discount factor  $\rho \in (0, 1)$ . In the MHE literature, the application of discounting in the disturbance terms has been introduced in [25] and has been proven to be particularly useful for various MHE stability results, compare [26]–[28]. It allows to obtain improved state estimation error bounds, as shown in the proof of Theorem 2 below. The cost function considers additionally the prior weighting, defined as

$$\Gamma(\bar{x}(t-L|t)) := |\bar{x}(t-L|t) - \hat{x}(t-L)|_P^2 \rho^L, \quad (8)$$

for a weighting matrix  $P$ . The prior weighting penalizes the difference between the estimated state at the beginning of the horizon, i.e.,  $\bar{x}(t-L|t)$ , and the prior estimate<sup>2</sup>  $\hat{x}(t-L)$  corresponding to the state estimate at time  $t-L$ . The prior weighting hence takes into account previous measurements that are not part of the current horizon. By means of the matrices  $R$  and  $P$ , we trade off how much we believe our measurements and how much we believe our prior.

At the beginning of the estimation, there are not enough measurements available to fill a complete horizon  $L$ . In that case, the data-driven MHE (6) is slightly adapted. Namely, for each time  $t < L$ , solve

$$\underset{\substack{\bar{x}_{[-t,0]}(t), \alpha(t), \\ \sigma_{[-t,-1]}^y(t)}}{\text{minimize}} \quad J_t(\bar{x}(0|t), \sigma_{[-t,-1]}^y(t)) \quad (9a)$$

$$\text{s. t.} \quad \begin{bmatrix} H_t(u_{[0,N-2]}^d) \\ H_t(y_{[0,N-2]}^d) \\ H_{t+1}(x_{[0,N-1]}^d) \end{bmatrix} \alpha(t) = \begin{bmatrix} u_{[0,t-1]} \\ \tilde{y}_{[0,t-1]} - \sigma_{[-t,-1]}^y(t) \\ \bar{x}_{[-t,0]}(t) \end{bmatrix} \quad (9b)$$

$$\bar{x}_{[-t,0]}(t) \in \mathbb{X} \quad (9c)$$

where

$$J_t(\bar{x}(0|t), \sigma_{[-t,-1]}^y(t)) := \Gamma(\bar{x}(0|t)) + \sum_{k=1}^t \ell_k(\sigma^y(t-k|t)) \quad (9d)$$

with  $\ell_k$  as defined in (7) and

$$\Gamma(\bar{x}(0|t)) := |\bar{x}(0|t) - \hat{x}(0)|_P^2 \rho^t. \quad (10)$$

Note that in this initial time interval, the dimensions of the Hankel matrices in (9b) change at every time instant, since the estimated trajectory lengths depend on the time instances.

*Remark 2:* This initial phase is treated by the so-called full information estimator (FIE), meaning that all available measurements are taken into account, as done in most model-based MHE schemes [23], [24]. Ideally, we would like to apply the FIE for all times  $t \geq L$ . However, as in the model-based case, the optimization problem becomes intractable because its size grows unboundedly as more and more measurements are considered [4]. Additionally, the application of the FIE for all times  $t \geq L$  would, in the limit, require an infinitely deep Hankel matrix and an input sequence which is persistently exciting of order infinity, which is impossible. This issue is specific to the data-driven MHE scheme and its implicit system representation; it does not occur in model-based MHE schemes.

*Remark 3:* In [20], the *filtering* form of MHE is used. This means that the most recent output measurement (i.e.,  $\tilde{y}(t)$ ) is taken into account when estimating  $\hat{x}(t)$ , compare problem (5) in [20]. Here, we employ the *prediction* form of MHE, i.e., in order to estimate the state at time  $t$ , we do not consider  $\tilde{y}(t)$ . This principle also explains the origin of the name: we *predict* the state at time  $t$ , based on output measurements up to time  $t-1$ . The application of the prediction form is possible since  $x(t)$  does not depend on  $u(t)$  and  $y(t)$ . The prediction form of MHE has better (less conservative) theoretical properties, whereas the filtering form of MHE typically performs better in practice, compare the discussion in [24]. For a more detailed explanation regarding the different forms of MHE, see, e.g., [24]. In the following proofs, the application of the prediction form of MHE leads to substantial simplifications compared to the filtering form of MHE. Nevertheless, all of the following results can also be established for the filtering form of MHE, albeit with some additional (technical) steps in the proofs.

In the following, we prove RGES of the data-driven MHE scheme. To simplify the notation, we denote sequences of finite or infinite length by bold face symbols  $\mathbf{v} := \{v(t_1), \dots, v(t_2)\}$  for some  $t_1, t_2 \in \mathbb{I}_{\geq 0}$  or  $\mathbf{v} := \{v(t_1), v(t_1+1), \dots\}$ . The length of these sequences will be understood from the context. The solution to (5) at time  $t$  for initial condition  $x_0$  and input sequence  $\mathbf{u}$  is denoted by  $x(t; x_0, \mathbf{u})$ . We denote the corresponding output as  $y(t) = Cx(t) + Du(t) =: h(x(t; x_0, \mathbf{u}), u(t))$ .

In order to prove RGES, we will assume (compare Assumption 2 below) that the considered system (5) is detectable, which implies “incremental exponential uniform output-to-state stability” (e-UOSS) [29, Corollary 7], [3] as defined below.

*Definition 2:* The linear system (5) is e-UOSS if there exist constants  $p_0, r_0 \geq 1$ ,  $\eta \in (0, 1)$  such that for each pair of initial conditions  $x_1, x_2 \in \mathbb{R}^n$  and any input sequence  $\mathbf{u}$  generating the states  $x(t; x_1, \mathbf{u})$  and  $x(t; x_2, \mathbf{u})$  the following holds

<sup>2</sup>This prior is typically called “filtering prior” in the MHE literature, compare, e.g., [24].

for all  $t \in \mathbb{I}_{\geq 0}$ :

$$|x(t; x_1, \mathbf{u}) - x(t; x_2, \mathbf{u})| \leq p_0 |x_1 - x_2| \eta^t + \sum_{\tau=1}^t r_0 |h(x(t-\tau; x_1, \mathbf{u}), u(t-\tau)) - h(x(t-\tau; x_2, \mathbf{u}), u(t-\tau))| \eta^\tau. \quad (11)$$

The notion of “uniformity” is used since the right-hand side of (11) holds uniformly for all  $\mathbf{u}$  (with the same  $p_0$ ,  $r_0$ , and  $\eta$ ). Compared to [20], we consider a definition of e-UOSS that considers discounting in the term related to the nominal output of the system. Furthermore, we replace the max-operator formulation with a sum-based formulation, since the latter allows to exploit Jensen’s inequality [30] in the subsequent analysis, which leads to less conservative state estimation error bounds. Note that this inequality has also been used in the model-based MHE context to improve state estimation error bounds, compare [28].

*Remark 4:* In many model-based MHE stability proofs, the notion of incremental input/output-to-state stability (i-IOSS) is employed. The e-UOSS property considered here differs from that notion by (i) using the exponential version which is always satisfied for linear detectable systems (compare, e.g., [29, Corollary 7]) and by (ii) only considering an output term in (11), but not an additional disturbance input. The extension of our results to this additional disturbance input (also referred to as process noise) is an interesting issue for future research, compare also Remark 5 in Section IV.

In what follows, we will prove RGES of the data-driven MHE in the sense of the following definition.

*Definition 3:* Consider system (5), subject to a disturbance  $v \in \mathbb{V}$ . A state estimator is RGES if there exist constants  $c_1$ ,  $c_2 \geq 1$  and  $\lambda_1, \lambda_2 \in (0, 1)$  such that for all  $x_0, \hat{x}(0) \in \mathbb{R}^n$ , and all  $v \in \mathbb{V}$ , the following is satisfied for all  $t \in \mathbb{I}_{\geq 0}$ :

$$|x(t) - \hat{x}(t)| \leq c_1 |x_0 - \hat{x}(0)| \lambda_1^t + \sum_{\tau=1}^t c_2 |v(t-\tau)| \lambda_2^\tau. \quad (12)$$

In order to prove RGES, we need the following three standard assumptions.

*Assumption 1:* The considered system (5) is controllable and the offline collected input  $\{u^d(k)\}_{k=0}^{N-1}$  is persistently exciting of order  $L + n + 1$ .

*Assumption 2:* The pair  $(A, C)$  of system (5) is detectable and the discount factor  $\rho$  in (7), (8), and (10) is selected such that  $\eta \leq \rho$ , for  $\eta$  in (11).

The assumption on the relation of the discount factors is needed for technical reasons that become clear in the proof of Theorem 2 below.

Recall the definitions of the stage costs  $\ell_k$  in (7) and of the prior weighting  $\Gamma$  in (8) and (10). Note that the quadratic expressions in the definitions of the stage costs and the prior weighting can always be lower bounded if the matrices  $R$  and  $P$  are positive definite, i.e.,  $r_1 |\sigma^y(t-\tau|t)|^2 \rho^k \leq |\sigma^y(t-\tau|t)|_R^2 \rho^k$  and  $p_1 |\bar{x}(t-L|t) - \hat{x}(t-L)|^2 \rho^L \leq |\bar{x}(t-L|t) - \hat{x}(t-L)|_P^2 \rho^L$  with  $r_1 := \lambda_{\min}(R)$  and  $p_1 := \lambda_{\min}(P)$ , respectively.

*Assumption 3:* The matrices  $R$  in (7) and  $P$  in (8), (10) are positive definite. Furthermore, it holds that  $p_0 \leq p_1$  and  $r_0 \leq r_1$  with  $p_0$  and  $r_0$  as from Definition 2.

In order to satisfy Assumptions 2 and 3, the constants  $r_0$ ,  $p_0$ , and  $\eta$  from Definition 2 need to be known. In Appendix A, we briefly outline how these can be computed in a data-driven fashion.

The following theorem was originally proven in the preliminary conference version [20]. However, in this work, we substantially improve the obtained state estimation error bounds by exploiting a discounted version of e-UOSS and Jensen’s inequality. Furthermore, in our current approach, the state estimation error bounds are uniformly bounded<sup>3</sup> in  $L$ . Finally, we simplify the proof by considering the prediction form of MHE instead of the filtering form of MHE that was considered in [20]. The proof technique will also be applied for the subsequent robust case.

*Theorem 2: (RGES of MHE)* Suppose Assumptions 1 - 3 hold. Then, there exists  $L_{\min}$  such that if  $L \geq L_{\min}$ , the MHE scheme defined in (6) and (9) is RGES, i.e., there exist  $c_1, c_2 \geq 1$  and  $\lambda_1, \lambda_2 \in (0, 1)$  such that for all  $x_0, \hat{x}(0) \in \mathbb{R}^n$  and for all  $t \in \mathbb{I}_{\geq 0}$ , (12) is satisfied.

The proof follows similar steps as the robust stability proofs of various model-based MHE schemes, see [23], [25], [27]. In turn, suitable adaptations to the data-driven setting are necessary such as, e.g., a representation of the system trajectories in a data-driven fashion and several simplifications due to the considered linear system.

**Proof:** First, we consider the optimal value function for  $t < L$ . A lower bound of the optimal value function can be found by exploiting Assumption 3 as follows,

$$\begin{aligned} J^*(\hat{x}(0|t), \hat{\sigma}_{[-t, -1]}^y(t)) \\ \geq p_0 |\hat{x}(0|t) - \hat{x}(0)|^2 \rho^t + r_0 \sum_{\tau=1}^t |\hat{\sigma}^y(t-\tau|t)|^2 \rho^\tau, \end{aligned} \quad (13)$$

<sup>3</sup>Due to the considered proof technique in [20], the state estimation error bounds deteriorate for an increasing horizon length  $L$ .

where  $J^*$  denotes the optimal value function. The application of Jensen's inequality [30] yields

$$J^*(\hat{x}(0|t), \hat{\sigma}_{[-t, -1]}^y(t)) \geq \left( p_0 \rho^t + r_0 \sum_{\tau=1}^t \rho^\tau \right)^{-1} \times \left( p_0 |\hat{x}(0|t) - \hat{x}(0)| \rho^t + r_0 \sum_{\tau=1}^t |\hat{\sigma}^y(t - \tau|t)| \rho^\tau \right)^2. \quad (14)$$

We define

$$c_J(t) := p_0 \rho^t + r_0 \sum_{\tau=1}^t \rho^\tau = p_0 \rho^t + r_0 \frac{\rho - \rho^{t+1}}{1 - \rho}. \quad (15)$$

The introduced variable is now used to reformulate (14) as

$$\sqrt{c_J(t) J^*} \geq p_0 |\hat{x}(0|t) - \hat{x}(0)| \rho^t + r_0 \sum_{\tau=1}^t |\hat{\sigma}^y(t - \tau|t)| \rho^\tau. \quad (16)$$

Next, we upper bound the optimal value function by a candidate trajectory which is chosen as the real (unknown) system trajectory that we want to observe. This trajectory starts at  $x(0) = x_0$  and is corrupted by the real measurement noise  $v$ . The costs associated with this trajectory are

$$\begin{aligned} J^*(\hat{x}(0|t), \hat{\sigma}_{[-t, -1]}^y(t)) &\leq J(x(0), v_{[0, t-1]}) \\ &\leq p_2 |x(0) - \hat{x}(0)|^2 \rho^t + r_2 \sum_{\tau=1}^t |v(t - \tau)|^2 \rho^\tau, \end{aligned} \quad (17)$$

where  $p_2 := \lambda_{\max}(P)$  and  $r_2 := \lambda_{\max}(R)$ . In order to connect the established lower bound (16) with the upper bound (17), we multiply (17) by  $c_J(t)$  and take the square root. Furthermore, we exploit that  $\sqrt{a + b} \leq \sqrt{a} + \sqrt{b}$  for any positive constants  $a, b$ , hence

$$\begin{aligned} &\sqrt{c_J(t) J^*} \\ &\leq \sqrt{c_J(t) p_2 |x(0) - \hat{x}(0)|^2 \rho^t + c_J(t) r_2 \sum_{\tau=1}^t |v(t - \tau)|^2 \rho^\tau} \\ &\leq \sqrt{c_J(t) p_2} |x(0) - \hat{x}(0)| \rho^{t/2} \\ &\quad + \sqrt{c_J(t) r_2} \sum_{\tau=1}^t |v(t - \tau)| \rho^{\tau/2}. \end{aligned} \quad (18)$$

We finalize these first considerations by combining the bounds derived in (16) and (18), leading to

$$\begin{aligned} p_0 |\hat{x}(0|t) - \hat{x}(0)| \rho^t + r_0 \sum_{\tau=1}^t |\hat{\sigma}^y(t - \tau|t)| \rho^\tau &\leq \sqrt{c_J(t) J^*} \\ &\leq \sqrt{c_J(t) p_2} |x(0) - \hat{x}(0)| \rho^{t/2} \\ &\quad + \sqrt{c_J(t) r_2} \sum_{\tau=1}^t |v(t - \tau)| \rho^{\tau/2}. \end{aligned} \quad (19)$$

Second, since the pair  $(A, C)$  is detectable by Assumption 2, system (5) is e-UOSS, compare [29, Corollary 7]. We apply this e-UOSS property with the following pair of trajectories: first, we use again the real (unknown) system trajectory that starts at  $x_1 = x(0)$ . Second, we use the estimated system trajectory starting at  $x_2 = \hat{x}(0|t)$ . Regarding the real unknown state trajectory of system (5), it follows, by applying the fundamental lemma (see (3) with  $y = x$ ) (and since we consider systems without process disturbances) that there exists an unknown  $\alpha$  such that

$$x(t) = x(t; x_1, \mathbf{u}) = H_1(x_{[t, N-1]}^d) \alpha(t),$$

with  $N$  denoting the number of collected data samples. Furthermore, by the definition of the estimated state  $\hat{x}$ , it holds that

$$\hat{x}(t) = x(t; x_2, \mathbf{u}) = H_1(x_{[t, N-1]}^d) \hat{\alpha}(t),$$

where we recall that  $\hat{\alpha}$  is the optimizer to problem (9). Additionally, for all  $\tau \leq t$ , we have that  $h(x(t-\tau; x_1, \mathbf{u}), u(t-\tau)) = H_1(y_{[t-\tau, N-1-\tau]}^d) \alpha(t) = \tilde{y}(t-\tau) - v(t-\tau)$  and  $h(x(t-\tau; x_2, \mathbf{u}), u(t-\tau)) = H_1(y_{[t-\tau, N-1-\tau]}^d) \hat{\alpha}(t) = \tilde{y}(t-\tau) - \hat{\sigma}^y(t-\tau|t)$ , leading to

$$\begin{aligned}
 |x(t) - \hat{x}(t)| &\leq p_0 |x(0) - \hat{x}(0)| \eta^t \\
 &\quad + \sum_{\tau=1}^t r_0 |h(x(t-\tau; x_1, \mathbf{u}), u(t-\tau)) \\
 &\quad \quad - h(x(t-\tau; x_2, \mathbf{u}), u(t-\tau))| \eta^\tau \\
 &= p_0 |x(0) - \hat{x}(0)| \eta^t \\
 &\quad + \sum_{\tau=1}^t r_0 |v(t-\tau) - \hat{\sigma}^y(t-\tau|t)| \eta^\tau \\
 &\leq p_0 |x(0) - \hat{x}(0)| \eta^t + p_0 |\hat{x}(0) - \hat{x}(0)| \eta^t \\
 &\quad + \sum_{\tau=1}^t r_0 |v(t-\tau)| \eta^\tau + \sum_{\tau=1}^t r_0 |\hat{\sigma}^y(t-\tau|t)| \eta^\tau.
 \end{aligned} \tag{20}$$

Now we make use of the derived bounds in (19). Namely, by Assumption 2, the second and the fourth term of (20) can be upper bounded by the left-hand side expression of (19) and, therefore, we get

$$\begin{aligned}
 |x(t) - \hat{x}(t)| &\leq p_0 |x(0) - \hat{x}(0)| \eta^t + \sum_{\tau=1}^t r_0 |v(t-\tau)| \eta^\tau \\
 &\quad + \sqrt{c_J(t) p_2} |x(0) - \hat{x}(0)| \rho^{t/2} \\
 &\quad + \sqrt{c_J(t) r_2} \sum_{\tau=1}^t |v(t-\tau)| \rho^{\tau/2}.
 \end{aligned} \tag{21}$$

Defining  $\lambda := \rho^{1/2}$  and using the fact that Assumption 2 implies  $\eta \leq \rho^{1/2} = \lambda$ , we simplify

$$|x(t) - \hat{x}(t)| \leq P_0 |x(0) - \hat{x}(0)| \lambda^t + \sum_{\tau=1}^t R_0 |v(t-\tau)| \lambda^\tau \tag{22}$$

with

$$P_0 := p_0 + \sqrt{c_J(0) p_2}, \tag{23}$$

$$R_0 := r_0 + \sqrt{c_J(0) r_2}, \tag{24}$$

since  $c_J(t+1) < c_J(t) \ \forall t \in \mathbb{I}_{\geq 0}$  when  $\rho < \frac{p_0}{p_0 + r_0}$  (compare the reasoning in Appendix B), which can always be satisfied by choosing  $p_0$  large enough. Whenever  $\rho > \frac{p_0}{p_0 + r_0}$ , it holds that  $c_J(t) < c_J(t+1) \ \forall t \in \mathbb{I}_{\geq 0}$ . In this case, one can set  $P_0 = p_0 + \sqrt{c_J(L) p_2}$  and  $R_0 = r_0 + \sqrt{c_J(L) r_2}$ . The derived expression (22) holds for all  $t < L$ . Since we use a filtering prior (meaning that we use  $\hat{x}(t-L)$  in the definition of the prior weighting, compare (8)), we can reformulate this result for all  $t \geq L$  as

$$\begin{aligned}
 |x(t) - \hat{x}(t)| &\leq P_0 |x(t-L) - \hat{x}(t-L)| \lambda^L \\
 &\quad + \sum_{\tau=1}^L R_0 |v(t-\tau)| \lambda^\tau.
 \end{aligned} \tag{25}$$

From here on, we can use similar ideas<sup>4</sup> as in [23], [27] to obtain the desired result. We choose an  $L$  large enough, so  $\mu = P_0 \lambda^L \in (0, 1)$ . This is possible, since  $P_0$  is bounded as  $L \rightarrow \infty$  and since  $\lambda \in (0, 1)$ . Hence, we establish a contraction from time  $t-L$  up to time  $t$  and get

$$\begin{aligned}
 |x(t) - \hat{x}(t)| &\leq \mu |x(t-L) - \hat{x}(t-L)| \\
 &\quad + R_0 \sum_{\tau=1}^L |v(t-\tau)| \lambda^\tau.
 \end{aligned} \tag{26}$$

<sup>4</sup>The main difference is that we only consider measurement noise but no process noise.

We apply this bound recursively using  $t = TL + \tilde{t}$  with  $T \in \mathbb{N}, \tilde{t} \in \mathbb{I}_{[0, L-1]}$ . Loosely speaking,  $T$  is the number of horizons that have been filled at time  $t$ . Hence, we obtain

$$\begin{aligned} |x(t) - \hat{x}(t)| &\leq \mu^T |x(t - TL) - \hat{x}(t - TL)| \\ &\quad + R_0 \sum_{k=0}^{T-1} \mu^k \sum_{\tau=1}^L |v(t - kL - \tau)| \lambda^\tau. \end{aligned} \quad (27)$$

Note that  $t - TL = \tilde{t} \in \mathbb{I}_{[0, L-1]}$ . Therefore, we can make use of (22) to replace the first term of (27), resulting in

$$\begin{aligned} |x(t) - \hat{x}(t)| &\leq \mu^T (P_0 |x(0) - \hat{x}(0)| \lambda^{\tilde{t}} + R_0 \sum_{\tau=1}^{\tilde{t}} |v(\tilde{t} - \tau)| \lambda^\tau) \\ &\quad + R_0 \sum_{k=0}^{T-1} \mu^k \sum_{\tau=1}^L |v(t - kL - \tau)| \lambda^\tau \\ &= \mu^T P_0 |x(0) - \hat{x}(0)| \lambda^{\tilde{t}} + \mu^T R_0 \sum_{\tau=1}^{\tilde{t}} |v(\tilde{t} - \tau)| \lambda^\tau \\ &\quad + R_0 \sum_{k=0}^{T-1} \mu^k \sum_{\tau=1}^L |v(t - kL - \tau)| \lambda^\tau \end{aligned} \quad (28)$$

Define  $\tilde{\lambda} = \mu^{\frac{1}{L}} \in (0, 1)$  (which implies  $\tilde{\lambda} \geq \lambda$ , because  $\tilde{\lambda} = \mu^{\frac{1}{L}} = (P_0 \lambda^L)^{\frac{1}{L}} = P_0^{\frac{1}{L}} \lambda \geq \lambda$ , since  $P_0 \geq 1$ ). Note that  $\mu^T \lambda^{\tilde{t}} \leq \mu^T \tilde{\lambda}^{\tilde{t}} = \mu^T \mu^{\frac{\tilde{t}}{L}} = \mu^{\frac{TL + \tilde{t}}{L}} = \mu^{\frac{t}{L}} = \tilde{\lambda}^t$ . Similarly, we obtain  $\mu^T \lambda^\tau \leq \tilde{\lambda}^{TL + \tau}$  as well as  $\mu^k \lambda^\tau \leq \tilde{\lambda}^{kL + \tau}$ . This yields

$$\begin{aligned} |x(t) - \hat{x}(t)| &\leq P_0 |x(0) - \hat{x}(0)| \tilde{\lambda}^t \\ &\quad + R_0 \tilde{\lambda}^{TL} \sum_{\tau=1}^{\tilde{t}} |v(\tilde{t} - \tau)| \tilde{\lambda}^\tau \\ &\quad + R_0 \sum_{k=0}^{T-1} \tilde{\lambda}^{kL} \sum_{\tau=1}^L |v(t - kL - \tau)| \tilde{\lambda}^\tau, \end{aligned} \quad (29)$$

The aim is now to bring equation (29) into the desired form (12). The first term of inequality (29) is already in the correct form. The second term can be reformulated by

$$R_0 \tilde{\lambda}^{TL} \sum_{\tau=1}^{\tilde{t}} |v(\tilde{t} - \tau)| \tilde{\lambda}^\tau = R_0 \sum_{\tau=1}^{\tilde{t}} |v(\tilde{t} - \tau)| \tilde{\lambda}^{\tau + TL}. \quad (30)$$

The third term of equation (29) can be reformulated as follows

$$R_0 \sum_{k=0}^{T-1} \tilde{\lambda}^{kL} \sum_{\tau=1}^L |v(t - kL - \tau)| \tilde{\lambda}^\tau = R_0 \sum_{\tau=1}^{TL} |v(t - \tau)| \tilde{\lambda}^\tau. \quad (31)$$

Now we sum up the right-hand sides of equations (30) and (31) and obtain

$$\begin{aligned} &R_0 \sum_{\tau=1}^{\tilde{t}} |v(\tilde{t} - \tau)| \tilde{\lambda}^{\tau + TL} + R_0 \sum_{\tau=1}^{TL} |v(t - \tau)| \tilde{\lambda}^\tau \\ &= R_0 \sum_{\tau=1}^t |v(t - \tau)| \tilde{\lambda}^\tau. \end{aligned} \quad (32)$$

Finally, we can reformulate (29) using (32) and obtain

$$|x(t) - \hat{x}(t)| \leq P_0 |x(0) - \hat{x}(0)| \tilde{\lambda}^t + R_0 \sum_{\tau=1}^t |v(t - \tau)| \tilde{\lambda}^\tau, \quad (33)$$

which proves RGES of the data-driven MHE scheme. ■

This proof technique improves substantially the preliminary results shown in [20] by (i) exploiting Jensen's inequality and by (ii) working with a discounted version of the e-UOSS property. Consequently, the state estimation error bounds are (much) less conservative *and* the obtained bounds are independent of the horizon length  $L$  for  $\rho < \frac{p_0}{p_0 + r_0}$ , compare the detailed explanation of this relation in Appendix B. Please note that this inequality can always be satisfied by choosing  $p_0$  large enough. In any



case, and independent whether or not  $\rho$  satisfies the above inequality<sup>5</sup>, the state estimation error bounds are uniformly bounded in  $L$ . In contrast to [20], the here derived state estimation error bounds do *not* grow unboundedly as  $L \rightarrow \infty$ . However, we still need a minimum horizon length  $L$  to establish a contraction mapping and hence to prove RGES.

Note that the final decrease rate is

$$\tilde{\lambda} = \mu^{1/L} = (P_0 \lambda^L)^{1/L} = P_0^{1/L} \lambda = P_0^{1/L} \rho^{1/2}, \quad (34)$$

where  $\rho$  is the discount factor of the cost function. Therefore, even if we chose  $\rho = \eta$  and let  $L \rightarrow \infty$ , the final decrease rate would correspond to  $\eta^{1/2}$ , which is a worse decrease rate than  $\eta$  (the constant from the e-UOSS condition, see Definition 2), since  $\eta \in (0, 1)$ . This result is unavoidable when using this proof technique, since the cost function (6d) contains quadratic terms, while the e-UOSS property (11) contains norms (and not quadratic terms).

Recently, in the context of model-based MHE, a Lyapunov-based proof has been proposed to show RGES in [31], which resulted in an even smaller minimum horizon length to guarantee RGES. Investigating whether this proof technique can also be applied to the data-driven setting and how it potentially improves the minimum horizon length is subject of ongoing research.

#### IV. PRACTICAL RES FOR NOISY OFFLINE STATE & OUTPUT MEASUREMENTS

In this section, we relax the data-driven MHE setup by allowing the offline collected output and state measurements to be corrupted by some persistent but bounded noise. That is, we can only measure the noisy a priori data

$$\tilde{y}^d(t) = y^d(t) + \varepsilon_y^d(t) \quad (35)$$

$$\tilde{x}^d(t) = x^d(t) + \varepsilon_x^d(t), \quad (36)$$

where  $\varepsilon_x^d$  and  $\varepsilon_y^d$  are the offline state and output measurement noise with  $|\varepsilon_x^d(t)|_\infty \leq \bar{\varepsilon}_x^d$  and  $|\varepsilon_y^d(t)|_\infty \leq \bar{\varepsilon}_y^d$ , respectively. Furthermore, we define

$$\bar{\varepsilon}^d := \max\{\bar{\varepsilon}_y^d, \bar{\varepsilon}_x^d\}. \quad (37)$$

The data-driven MHE scheme needs to be adapted in the following way. At each time  $t \geq L$ , solve

$$\begin{aligned} & \underset{\substack{\bar{x}_{[-L,0]}(t), \alpha(t), \\ \sigma_{[-L,-1]}^y(t), \\ \sigma_{[-L,0]}^x(t)}}{\text{minimize}} & J(\bar{x}(t-L|t), \sigma_{[-L,-1]}^y(t), \sigma_{[-L,0]}^x(t), \alpha(t)) \end{aligned} \quad (38a)$$

$$\text{s. t.} \quad \begin{bmatrix} H_L(u_{[0,N-2]}^d) \\ H_L(\tilde{y}_{[0,N-2]}^d) \\ H_{L+1}(\tilde{x}_{[0,N-1]}^d) \end{bmatrix} \alpha(t) = \begin{bmatrix} u_{[t-L,t-1]} \\ \tilde{y}_{[t-L,t-1]} - \sigma_{[-L,-1]}^y(t) \\ \bar{x}_{[-L,0]}(t) + \sigma_{[-L,0]}^x(t) \end{bmatrix} \quad (38b)$$

$$\bar{x}_{[-L,0]}(t) \in \mathbb{X} \quad (38c)$$

where

$$\begin{aligned} & J(\bar{x}(t-L|t), \sigma_{[-L,-1]}^y(t), \sigma_{[-L,0]}^x(t), \alpha(t)) \\ & := \Gamma(\bar{x}(t-L|t)) + \sum_{k=1}^L \ell_k(\sigma^y(t-k|t)) \\ & + c_{\sigma^x} |\sigma_{[-L,0]}^x(t)|^2 + c_\alpha (\bar{\varepsilon}_x^d + \bar{\varepsilon}_y^d) |\alpha(t)|^2 \end{aligned} \quad (38d)$$

for  $c_{\sigma^x} \geq p_0$  and  $c_\alpha \geq \max\{\frac{\eta-\eta^{L+1}}{1-\eta} r_0 \sqrt{p}(N-1), 2p_0 \sqrt{nN}\}$ . The minimal values of  $c_{\sigma^x}$  and  $c_\alpha$  are necessary to establish pRES as shown in the following proof. Here, the online estimated state trajectory  $\bar{x}_{[-L,0]}(t)$  is a linear combination of time-shifts of a noisy offline state trajectory. In comparison with (6), this requires an additional slack variable  $\sigma^x$  in the last block row of (38b). Without  $\sigma^x$ , we could not guarantee that the estimated state sequence respects the constraints (38c). The cost function considers two additional quadratic regularization terms. The first one is related to  $\sigma^x$ , which is incorporated to bring the solution closer to the span of the noisy collected state sequence. The second one is related to  $\alpha$ , and is needed to limit the amplification of the noise affecting the offline collected data. Regularizations are particularly common in the dual problem of data-driven MPC, compare [11], [12], [32]. Note that for the nominal introduced data-driven MHE scheme (6), no regularization term for  $\alpha$  is included in the cost function, see definitions (6d) and (9d). This is due to the setting in the previous section, where we consider that the offline state and output measurements are noise-free and hence  $\alpha$  cannot amplify any noise in the offline data. The optimizers of problem (38) are denoted by  $\hat{x}_{[-L,0]}(t)$ ,  $\hat{\sigma}_{[-L,-1]}^y(t)$ ,  $\hat{\sigma}_{[-L,0]}^x(t)$ , and  $\alpha(t)$ . Once again, the state estimate at time  $t$  is defined as  $\hat{x}(t) := \hat{x}(t|t)$ .

<sup>5</sup>For  $\rho > \frac{p_0}{p_0+r_0}$  the derived bounds increase for an increasing horizon length  $L$ , but are also uniformly bounded in  $L$ .

The stage costs and the prior weighting are defined as in (7) and in (8), respectively. As long as one complete horizon is not filled, i.e., for  $t < L$ , we apply once again the FIE. The changes for robust data-driven FIE compared to the robust data-driven MHE scheme (38) are completely analogous to the previous section. For the sake of brevity, these changes are not shown here.

In order to show pRES of the introduced data-driven MHE (38), we need one further assumption.

**Assumption 4:** The inputs  $u$  and the states  $x$  of the considered system (5) evolve in compact sets  $\mathbb{U}$  and  $\tilde{\mathbb{X}}$ , i.e.,  $u(t) \in \mathbb{U}$  and  $x(t) \in \tilde{\mathbb{X}}$ , respectively.

Assumption 4 implies that the states of system (5) do not grow unboundedly. If necessary, a pre-stabilizing controller can be applied to system (5) to ensure that Assumption 4 holds.

The main objective of this section is to show that the introduced robust data-driven MHE scheme in (38) is pRES with respect to the following definition.

**Definition 4:** Consider system (5) subject to disturbances  $v \in \mathbb{V}$ . Moreover, consider noisy a priori output and state measurements as defined in (35) and (36), respectively. A state estimator is pRES if there exist constants  $c_1, c_2 \geq 1$ ,  $\lambda_1, \lambda_2 \in (0, 1)$  and a function  $\gamma \in \mathcal{K}$  such that for all  $x_0, \hat{x}(0) \in \tilde{X}$ , all  $v \in \mathbb{V}$ , and all  $\bar{\varepsilon}_x^d, \bar{\varepsilon}_y^d \geq 0$  the following is satisfied for all  $t \in \mathbb{I}_{\geq 0}$ :

$$\begin{aligned} & |x(t) - \hat{x}(t)| \\ & \leq c_1 |x_0 - \hat{x}(0)| \lambda_1^t + \sum_{\tau=0}^t c_2 |v(t - \tau)| \lambda_2^\tau + \gamma(\bar{\varepsilon}^d). \end{aligned} \quad (39)$$

Definition 4 states that we can upper bound the differences between the true (unknown) states and the estimated states by means of (i) their difference in the initial conditions (ii) the true measurement noise affecting the online output measurements and (iii) a  $\mathcal{K}$  function depending on  $\bar{\varepsilon}^d$  in (37). Recall that since  $\gamma \in \mathcal{K}$ , we have  $\gamma(0) = 0$ , meaning that we recover Definition 3 when the measurements in the offline phase are noise-free. Furthermore, this definition states that smaller values for  $\bar{\varepsilon}^d$  imply smaller state estimation error bounds. The main result of this paper is given by the following theorem.

**Theorem 3:** (pRES of robust MHE) Consider system (5) subject to noise  $\varepsilon_x^d$  and  $\varepsilon_y^d$  in the (offline) data collection phase and to  $v \in \mathbb{V}$  in the online phase. Let Assumptions 1 - 4 hold. Then, there exists  $L_{\min}$  such that for all  $L > L_{\min}$  the robust data-driven MHE scheme (38) is pRES, i.e., there exist  $c_1, c_2 \geq 1$ ,  $\lambda_1, \lambda_2 \in (0, 1)$ , and a function  $\gamma \in \mathcal{K}$ , such that for all  $x_0, \hat{x}(0) \in \tilde{X}$ , all  $u \in \mathbb{U}$ , and for all  $t \in \mathbb{I}_{\geq 0}$ , (39) is satisfied.

**Proof:** The proof approach, i.e., combining lower and upper bounds of the cost function and relating them with the e-UOSS property to establish a contraction mapping, remains similar as in the proof of Theorem 2. However, there are many substantial changes necessary due to the considered noise in the offline collected outputs and states.

#### Part I: Establishment of a Contraction Mapping

In this part of the proof, we consider  $t < L$ . The first step is once again to lower bound the optimal value function (exploiting Assumption 3) for  $t < L$  resulting in

$$\begin{aligned} & J^*(\hat{x}(0|t), \hat{\sigma}_{[-t, -1]}^y(t), \hat{\sigma}_{[-t, 0]}^x(t), \hat{\alpha}(t)) \\ & \geq p_0 |\hat{x}(0) - \hat{x}(0|t)|^2 \rho^t + r_0 \sum_{\tau=1}^t |\hat{\sigma}^y(t - \tau|t)|^2 \rho^\tau \\ & \quad + c_{\sigma^x} |\hat{\sigma}_{[-t, 0]}^x(t)|^2 + c_\alpha (\bar{\varepsilon}_x^d + \bar{\varepsilon}_y^d) |\hat{\alpha}(t)|^2. \end{aligned}$$

Again, we apply Jensen's inequality

$$\begin{aligned} & J^*(\hat{x}(0|t), \hat{\sigma}_{[-t, -1]}^y(t), \hat{\sigma}_{[-t, 0]}^x(t), \hat{\alpha}(t)) \\ & \geq \left( p_0 \rho^t + r_0 \sum_{\tau=1}^t \rho^\tau + c_{\sigma^x} + c_\alpha (\bar{\varepsilon}_x^d + \bar{\varepsilon}_y^d) \right)^{-1} \times \\ & \quad \left( p_0 |\hat{x}(0) - \hat{x}(0|t)|^2 \rho^t + r_0 \sum_{\tau=1}^t |\hat{\sigma}^y(t - \tau|t)|^2 \rho^\tau \right. \\ & \quad \left. + c_{\sigma^x} |\hat{\sigma}_{[-t, 0]}^x(t)|^2 + c_\alpha (\bar{\varepsilon}_x^d + \bar{\varepsilon}_y^d) |\hat{\alpha}(t)|^2 \right). \end{aligned} \quad (40)$$

We define an auxiliary variable

$$\begin{aligned} c_{\bar{J}}(t, \bar{\varepsilon}_x^d, \bar{\varepsilon}_y^d) &:= p_0 \rho^t + r_0 \sum_{\tau=1}^t \rho^\tau + c_{\sigma^x} + c_\alpha (\bar{\varepsilon}_x^d + \bar{\varepsilon}_y^d) \\ &= p_0 \rho^t + r_0 \frac{\rho - \rho^{t+1}}{1 - \rho} + c_{\sigma^x} + c_\alpha (\bar{\varepsilon}_x^d + \bar{\varepsilon}_y^d). \end{aligned} \quad (41)$$

The introduced variable is now used to reformulate (40)

$$\begin{aligned} (c_{\bar{J}}(t, \bar{\varepsilon}_x^d, \bar{\varepsilon}_y^d) J^*)^{1/2} &\geq p_0 |\hat{x}(0) - \hat{x}(0|t)| \rho^t \\ &+ r_0 \sum_{\tau=1}^t |\hat{\sigma}^y(t - \tau|t)| \rho^\tau + c_{\sigma^x} |\hat{\sigma}_{[-t,0]}^x(t)| \\ &+ c_\alpha (\bar{\varepsilon}_x^d + \bar{\varepsilon}_y^d) |\hat{\alpha}(t)|. \end{aligned} \quad (42)$$

Next, we upper bound the optimal value function by means of a candidate trajectory. Here we exploit the following candidate trajectory. We choose  $\alpha(t)$  such that

$$\begin{bmatrix} H_t(u_{[0,N-2]}^d) \\ H_1(x_{[0,N-t-1]}^d) \end{bmatrix} \alpha(t) = \begin{bmatrix} u_{[0,t-1]} \\ x(0) \end{bmatrix}, \quad (43)$$

where  $x(0)$  denotes the real (unknown) system state  $x$  at time  $t = 0$  and  $u_{[0,t-1]}$  the real input sequence from time 0 up to  $t - 1$ . Please note that the left-hand side of (43) contains the (unknown) *noise-free* offline state sequence. According to Assumption 1 and Lemma 1, the concatenated Hankel matrices in equation (43) have full row rank. Therefore, there exists a right inverse (denoted by  $\dagger$ ) so that

$$\alpha(t) = \begin{bmatrix} H_t(u_{[0,N-2]}^d) \\ H_1(x_{[0,N-t-1]}^d) \end{bmatrix}^\dagger \begin{bmatrix} u_{[0,t-1]} \\ x(0) \end{bmatrix}. \quad (44)$$

The states and outputs of a DT-LTI system are linear combinations of the initial condition and the inputs (compare [9] for a detailed explanation), therefore the above choice of  $\alpha$  implies

$$\begin{bmatrix} H_t(u_{[0,N-2]}^d) \\ H_t(y_{[0,N-2]}^d) \\ H_{t+1}(x_{[0,N-1]}^d) \end{bmatrix} \alpha(t) = \begin{bmatrix} u_{[0,t-1]} \\ \tilde{y}_{[0,t-1]} - v_{[0,t-1]} \\ x_{[0,t]} \end{bmatrix}, \quad (45)$$

meaning that the real input, output, and state sequences are generated by that choice of  $\alpha$ , where we need to subtract the true measurement noise from the noisy output measurements in the second row of (45) in order to make Willems' lemma hold. The slack  $\sigma^x$  in relation to the candidate trajectory is chosen as

$$\sigma_{[-t,0]}^x(t) = H_{t+1}(\varepsilon_{x,[0,N-1]}^d) \alpha(t). \quad (46)$$

The slack  $\sigma^y$  must compensate the measurement noise (that occurs in the online phase) but also the noise affecting the offline collected output measurements. Therefore, the slack  $\sigma^y$  associated with the candidate trajectory is chosen as

$$\sigma_{[-t,-1]}^y(t) = \sigma_{[-t,-1]}^{\varepsilon_y}(t) + v_{[0,t-1]} \quad (47)$$

where  $v$  corresponds to the true measurement noise and

$$\sigma_{[-t,-1]}^{\varepsilon_y}(t) = H_t(\varepsilon_{y,[0,N-2]}^d) \alpha(t). \quad (48)$$

This selection of  $\alpha$ ,  $\sigma^x$  and  $\sigma^y$  implies that all constraints in (38b) are satisfied. Furthermore, (38c) holds since the real (undisturbed) state trajectory is contained in the constrained set  $\mathbb{X}$ . As in the previous section, we want to upper bound the cost function related to the candidate solution. Notice that, compared to (6a), the cost function in (38a) considers additional terms for which an upper bound is needed. First, we can bound  $|\alpha|$  by using (44) to obtain

$$|\alpha(t)| \leq \left\| \begin{bmatrix} H_t(u_{[0,N-2]}^d) \\ H_1(x_{[0,N-t-1]}^d) \end{bmatrix}^\dagger \right\| \left\| \begin{bmatrix} u_{[0,t-1]} \\ x(0) \end{bmatrix} \right\|. \quad (49)$$

Since  $u(t)$  and  $x(t)$  evolve in a compact set (according to Assumption 4), there exist a  $u_{\max}$  and an  $x_{\max}$  so that  $|u(t)| \leq u_{\max}$  and  $|x(t)| \leq x_{\max} \quad \forall t \in \mathbb{I}_{\geq 0}$ . Additionally, we define

$$H_{\text{ux}} := \left\| \begin{bmatrix} H_t(u_{[0,N-2]}^d) \\ H_1(x_{[0,N-t-1]}^d) \end{bmatrix}^\dagger \right\|. \quad (50)$$

In conclusion, it holds that

$$|\alpha(t)| \leq H_{\text{ux}}(Lu_{\max} + x_{\max}) =: \alpha_{\max}. \quad (51)$$

Hence, the variable  $\alpha(t)$  associated with the candidate solution is upper bounded at any time  $t$ . Now, to upper bound the slack defined in (46), we have

$$\begin{aligned} |\sigma_{[-t,0]}^x(t)| &\leq |H_{t+1}(\varepsilon_{x,[0,N-1]}^d)| |\alpha(t)| \\ &\leq |H_{t+1}(\varepsilon_{x,[0,N-1]}^d)| \alpha_{\max} =: \sigma_{\max}^x. \end{aligned} \quad (52)$$

Finally, an upper bound for  $\sigma_{[-t,-1]}^{\varepsilon_y}$  can be established by

$$\begin{aligned} |\sigma_{[-t,-1]}^{\varepsilon_y}(t)| &\leq |H_t(\varepsilon_{y,[0,N-2]}^d)| |\alpha(t)| \\ &\leq |H_t(\varepsilon_{y,[0,N-2]}^d)| \alpha_{\max} =: \sigma_{\max}^{\varepsilon_y} \end{aligned} \quad (53)$$

From here on, we consider the cost associated with the candidate trajectory defined by (43), (46), and (47). This candidate trajectory can be upper bounded by using the basic inequality  $(a+b)^2 \leq 2a^2 + 2b^2$  and Assumption 3

$$\begin{aligned} J^*(\hat{x}(0|t)) &\leq J(x(0)) \leq p_2 |\hat{x}(0) - x(0)|^2 \rho^t \\ &\quad + 2r_2 \sum_{\tau=1}^t |v(t-\tau)|^2 \rho^\tau + 2r_2 \sum_{\tau=1}^t |\sigma^{\varepsilon_y}(t-\tau|t)|^2 \rho^\tau \\ &\quad + c_{\sigma^x} |\sigma_{[-L,0]}^x(t)|^2 + c_\alpha (\bar{\varepsilon}_x^d + \bar{\varepsilon}_y^d) |\alpha(t)|^2. \end{aligned} \quad (54)$$

Note that we split the slack  $\sigma^y$  into  $v$  and  $\sigma^{\varepsilon_y}$ . In order to connect the established upper bound with the already derived lower bound, we need to multiply by  $c_{\bar{J}}(t, \bar{\varepsilon}_x^d, \bar{\varepsilon}_y^d)$  and to subsequently take the square root (using  $\sqrt{a+b} \leq \sqrt{a} + \sqrt{b}$  which holds for any  $a, b \geq 0$ ), yielding

$$\begin{aligned} &(c_{\bar{J}}(t, \bar{\varepsilon}_x^d, \bar{\varepsilon}_y^d) J^*(\hat{x}(0|t)))^{1/2} \\ &\leq \sqrt{c_{\bar{J}}(t, \bar{\varepsilon}_x^d, \bar{\varepsilon}_y^d) p_2} |\hat{x}(0) - x(0)| \rho^{t/2} \\ &\quad + \sqrt{c_{\bar{J}}(t, \bar{\varepsilon}_x^d, \bar{\varepsilon}_y^d) 2r_2} \sum_{\tau=1}^t |v(t-\tau)| \rho^{\tau/2} \\ &\quad + \sqrt{c_{\bar{J}}(t, \bar{\varepsilon}_x^d, \bar{\varepsilon}_y^d) 2r_2} \sum_{\tau=1}^t |\sigma^{\varepsilon_y}(t-\tau|t)| \rho^{\tau/2} \\ &\quad + \sqrt{c_{\bar{J}}(t, \bar{\varepsilon}_x^d, \bar{\varepsilon}_y^d) c_{\sigma^x}} |\sigma_{[-L,0]}^x(t)| \\ &\quad + \sqrt{c_{\bar{J}}(t, \bar{\varepsilon}_x^d, \bar{\varepsilon}_y^d) c_\alpha (\bar{\varepsilon}_x^d + \bar{\varepsilon}_y^d)} |\alpha(t)|. \end{aligned} \quad (55)$$

As in the previous section, we can combine the lower and the upper bound, namely

$$\text{RHS of (42)} \leq (c_{\bar{J}}(t, \bar{\varepsilon}_x^d, \bar{\varepsilon}_y^d) J^*(\hat{x}(0|t)))^{1/2} \leq \text{RHS of (55)}, \quad (56)$$

where the abbreviation RHS stands for “right-hand side”.

The second key ingredient to prove pRES of the robust data-driven MHE is to exploit the e-UOSS property. We here consider two trajectories. First, we consider the real (unknown) state trajectory parameterized by means of the candidate  $\alpha$ , compare (43). This real state trajectory starts at  $x_1 = x(0)$  and is driven by the input sequence  $\mathbf{u}$ . Its value at time  $t$  corresponds to  $x(t; x_1, \mathbf{u}) = x(t)$ . Second, we consider a state trajectory based on the estimated state sequence. We cannot choose exactly the estimated state sequence (as done in the previous section) since this sequence is not necessarily a valid system trajectory due to the considered noise in the offline phase. We consider a sequence starting at

$$\begin{aligned} x_2 &= \hat{x}(0|t) - H_1(\varepsilon_{x,[0,N-t-1]}^d) \hat{\alpha}(t) + \hat{\sigma}^x(0|t) \\ &= H_1(x_{[0,N-t-1]}^d) \hat{\alpha}(t), \end{aligned} \quad (57)$$

which can be deduced from the last row of (38b). After  $t$  time instances, the state value becomes

$$\begin{aligned} x(t; x_2, \mathbf{u}) &= \hat{x}(t) - H_1(\varepsilon_{x,[t,N-1]}^d) \hat{\alpha}(t) + \hat{\sigma}^x(t|t) \\ &= H_1(x_{[t,N-1]}^d) \hat{\alpha}(t). \end{aligned} \quad (58)$$

Therefore,

$$\begin{aligned} |x(t; x_1, \mathbf{u}) - x(t; x_2, \mathbf{u})| &= \\ &= |x(t) - \hat{x}(t) + H_1(\varepsilon_{x,[t,N-1]}^d) \hat{\alpha} - \hat{\sigma}^x(t|t)|. \end{aligned} \quad (59)$$

Note that  $|a| - |b| \leq |a - b|$ , which implies

$$\begin{aligned} |x(t) - \hat{x}(t)| &= | -H_1(\varepsilon_{x,[t,N-1]}^d)\hat{\alpha}(t) + \hat{\sigma}^x(t|t)| \\ &\leq |x(t) - \hat{x}(t) + H_1(\varepsilon_{x,[t,N-1]}^d)\hat{\alpha}(t) - \hat{\sigma}^x(t|t)| \\ &= |x(t; x_1, \mathbf{u}) - x(t; x_2, \mathbf{u})|. \end{aligned}$$

Reformulating the above inequality yields

$$\begin{aligned} |x(t) - \hat{x}(t)| &\leq |x(t; x_1, \mathbf{u}) - x(t; x_2, \mathbf{u})| \\ &\quad + | -H_1(\varepsilon_{x,[t,N-1]}^d)\hat{\alpha}(t) + \hat{\sigma}^x(t|t)|. \end{aligned}$$

Finally, we can replace the difference  $|x(t; x_1, \mathbf{u}) - x(t; x_2, \mathbf{u})|$  by means of the e-UOSS definition (11)

$$\begin{aligned} |x(t) - \hat{x}(t)| &\leq p_0|x(0) - \hat{x}(0|t) + H_1(\varepsilon_{x,[0,N-t-1]}^d)\hat{\alpha}(t) - \hat{\sigma}^x(0|t)|\eta^t \\ &\quad + \sum_{\tau=1}^t r_0|h(x(t-\tau; x_1, \mathbf{u}), u(t-\tau)) \\ &\quad \quad - h(x(t-\tau; x_2, \mathbf{u}), u(t-\tau))|\eta^\tau \\ &\quad + |H_1(\varepsilon_{x,[t,N-1]}^d)\hat{\alpha}(t)| + |\hat{\sigma}^x(t|t)|. \end{aligned} \quad (60)$$

In contrast to the nominal case,  $h(x(t-\tau; x_2, \mathbf{u}), u(t-\tau))$  no longer corresponds to  $\tilde{y}(t-\tau) - \hat{\sigma}^y(t-\tau|t)$ . However, we can establish the following relationship for  $0 \leq t \leq L-1$ , compare with the second row of (38b)

$$\begin{aligned} H_t(y_{[0,N-2]}^d)\hat{\alpha}(t) + H_t(\varepsilon_{y,[0,N-2]}^d)\hat{\alpha}(t) \\ = \tilde{y}_{[0,t-1]} - \hat{\sigma}_{[-t,-1]}^y(t). \end{aligned} \quad (61)$$

The expression for the nominal output trajectory (that is needed in the e-UOSS property) just corresponds to the first term of (61), namely  $H_t(y_{[0,N-2]}^d)\hat{\alpha}(t)$ . Therefore in the e-UOSS condition, we need to consider

$$\begin{aligned} \sum_{\tau=1}^t h(x(t-\tau; x_2, \mathbf{u}), u(t-\tau)) &= \sum_{\tau=1}^t H_1(y_{[t-\tau,N-1-\tau]}^d)\hat{\alpha}(t) \\ &= \sum_{\tau=1}^t (\tilde{y}(t-\tau) - \hat{\sigma}^y(t-\tau|t) - H_1(\varepsilon_{y,[t-\tau,N-1-\tau]}^d)\hat{\alpha}(t)). \end{aligned}$$

Therefore, (60) becomes

$$\begin{aligned} |x(t) - \hat{x}(t)| &\leq p_0|x(0) - \hat{x}(0|t) + H_1(\varepsilon_{x,[0,N-t-1]}^d)\hat{\alpha}(t) - \hat{\sigma}^x(0|t)|\eta^t \\ &\quad + \sum_{\tau=1}^t r_0|\tilde{y}(t-\tau) - v(t-\tau) \\ &\quad \quad - (\tilde{y}(t-\tau) - \hat{\sigma}^y(t-\tau|t) - H_1(\varepsilon_{y,[t-\tau,N-1-\tau]}^d)\hat{\alpha}(t))|\eta^\tau \\ &\quad + |H_1(\varepsilon_{x,[t,N-1]}^d)\hat{\alpha}(t)| + |\hat{\sigma}^x(t|t)| \\ &\leq p_0|\hat{x}(0) - x(0)|\eta^t + p_0|\hat{x}(0|t) - \hat{x}(0)|\eta^t \\ &\quad + \sum_{\tau=1}^t r_0|v(t-\tau)|\eta^\tau + \sum_{\tau=1}^t r_0|\hat{\sigma}^y(t-\tau|t)|\eta^\tau \\ &\quad + \sum_{\tau=1}^t r_0|H_1(\varepsilon_{y,[t-\tau,N-1-\tau]}^d)\hat{\alpha}(t)|\eta^\tau \\ &\quad + |H_1(\varepsilon_{x,[t,N-1]}^d)\hat{\alpha}(t)| + p_0|H_1(\varepsilon_{x,[0,N-t-1]}^d)\hat{\alpha}(t)| \\ &\quad + |\hat{\sigma}^x(t|t)| + p_0|\hat{\sigma}^x(0|t)|. \end{aligned} \quad (62)$$

Next, the aim is to combine (62) with the relation obtained in (56). This is possible since

$$p_0|\hat{x}(0|t) - \hat{x}(0)|\eta^t \leq p_0|\hat{x}(0) - \hat{x}(0|t)|\rho^t$$

and

$$r_0 \sum_{\tau=1}^t |\hat{\sigma}^y(t-\tau|t)|\eta^\tau \leq r_0 \sum_{\tau=1}^t r_0 |\hat{\sigma}^y(t-\tau|t)|\rho^\tau$$

by Assumption 2, as well as

$$\begin{aligned} |H_1(\varepsilon_{x,[t,N-1]}^d)\hat{\alpha}(t)| &\leq \sigma_{\max}(H_1(\varepsilon_{x,[t,N-1]}^d))|\hat{\alpha}(t)| \\ &\leq \|H_1(\varepsilon_{x,[t,N-1]}^d)\|_F |\hat{\alpha}(t)| \\ &= \sqrt{\sum_{i=1}^n \sum_{j=1}^{N-t} |\varepsilon_{x,i,j}^d|^2} |\hat{\alpha}(t)| \\ &\leq \sqrt{n(N-t)\bar{\varepsilon}_x^d} |\hat{\alpha}(t)| \\ &\leq \frac{1}{2} c_\alpha \bar{\varepsilon}_x^d |\hat{\alpha}(t)|, \end{aligned}$$

where  $\sigma_{\max}$  denotes the maximum singular value and  $\|\cdot\|_F$  the Frobenius norm. Similarly, we obtain

$$\begin{aligned} p_0 |H_1(\varepsilon_{x,[0,N-t-1]}^d)\hat{\alpha}(t)| &\leq p_0 \sqrt{n(N-t)\bar{\varepsilon}_x^d} |\hat{\alpha}(t)| \\ &\leq \frac{1}{2} c_\alpha \bar{\varepsilon}_x^d |\hat{\alpha}(t)|. \end{aligned}$$

Furthermore, it holds that

$$\begin{aligned} &\sum_{\tau=1}^t r_0 |H_1(\varepsilon_{y,[t-\tau,N-1-\tau]}^d)\hat{\alpha}(t)|\eta^\tau \\ &\leq \frac{\eta - \eta^{t+1}}{1 - \eta} r_0 \sqrt{p} |H_t(\varepsilon_{y,[0,N-2]}^d)|_\infty |\hat{\alpha}(t)| \\ &\leq \frac{\eta - \eta^{t+1}}{1 - \eta} r_0 \sqrt{p} (N-1) \bar{\varepsilon}_y^d |\hat{\alpha}(t)| \\ &\leq c_\alpha \bar{\varepsilon}_y^d |\hat{\alpha}(t)|. \end{aligned}$$

Finally, we can upper bound the last terms of (62) as

$$|\hat{\sigma}^x(t|t)| + p_0 |\hat{\sigma}^x(0|t)| \leq c_{\sigma^x} |\hat{\sigma}_{[-t,0]}^x(t)|$$

for  $c_{\sigma^x}$  from (38d). After combining the mentioned expressions, from (62) we get

$$\begin{aligned} |x(t) - \hat{x}(t)| &\leq p_0 |\hat{x}(0) - x(0)|\eta^t \\ &\quad + p_0 |\hat{x}(0) - \hat{x}(0|t)|\rho^t + \sum_{\tau=1}^t r_0 |v(t-\tau)|\eta^\tau \\ &\quad + r_0 \sum_{\tau=1}^t |\hat{\sigma}^y(t-\tau|t)|\rho^\tau \\ &\quad + c_\alpha (\bar{\varepsilon}_y^d + \bar{\varepsilon}_x^d) |\hat{\alpha}(t)| + c_{\sigma^x} |\hat{\sigma}_{[-t,0]}^x(t)|. \end{aligned} \tag{63}$$

Now, we exploit the established relation (56) to obtain

$$\begin{aligned} |x(t) - \hat{x}(t)| &\leq p_0 |\hat{x}(0) - x(0)|\eta^t + \sum_{\tau=1}^t r_0 |v(t-\tau)|\eta^\tau \\ &\quad + \sqrt{c_{\bar{j}}(t, \bar{\varepsilon}_x^d, \bar{\varepsilon}_y^d) p_2} |\hat{x}(0) - x(0)|\rho^{t/2} \\ &\quad + \sqrt{c_{\bar{j}}(t, \bar{\varepsilon}_x^d, \bar{\varepsilon}_y^d) 2r_2} \sum_{\tau=1}^t |v(t-\tau)|\rho^{\tau/2} \\ &\quad + \sqrt{c_{\bar{j}}(t, \bar{\varepsilon}_x^d, \bar{\varepsilon}_y^d) 2r_2} \sum_{\tau=1}^t |\sigma^{\varepsilon_y}(t-\tau|t)|\rho^{\tau/2} \\ &\quad + \sqrt{c_{\bar{j}}(t, \bar{\varepsilon}_x^d, \bar{\varepsilon}_y^d) c_\alpha (\bar{\varepsilon}_x^d + \bar{\varepsilon}_y^d)} |\alpha(t)| \\ &\quad + \sqrt{c_{\bar{j}}(t, \bar{\varepsilon}_x^d, \bar{\varepsilon}_y^d) c_{\sigma^x}} |\sigma_{[-t,0]}^x(t)| \end{aligned} \tag{64}$$

We define

$$\begin{aligned}\tilde{P}_0 &:= p_0 + \sqrt{c_{\tilde{J}}(t, \bar{\varepsilon}_x^d, \bar{\varepsilon}_y^d)} p_2, \\ \tilde{R}_0 &:= r_0 + \sqrt{c_{\tilde{J}}(t, \bar{\varepsilon}_x^d, \bar{\varepsilon}_y^d)} 2r_2, \\ \lambda &:= \rho^{1/2},\end{aligned}$$

and simplify inequality (64) as

$$\begin{aligned}|x(t) - \hat{x}(t)| &\leq \tilde{P}_0 |\hat{x}(0) - x(0)| \lambda^t + \sum_{\tau=1}^t \tilde{R}_0 |v(t - \tau)| \eta^\tau \\ &\quad + \sqrt{c_{\tilde{J}}(t, \bar{\varepsilon}_x^d, \bar{\varepsilon}_y^d)} 2r_2 \sum_{\tau=1}^t |\sigma^{\varepsilon_y}(t - \tau)| \lambda^\tau \\ &\quad + \sqrt{c_{\tilde{J}}(t, \bar{\varepsilon}_x^d, \bar{\varepsilon}_y^d)} c_\alpha (\bar{\varepsilon}_x^d + \bar{\varepsilon}_y^d) |\alpha(t)| \\ &\quad + \sqrt{c_{\tilde{J}}(t, \bar{\varepsilon}_x^d, \bar{\varepsilon}_y^d)} c_{\sigma^x} |\sigma_{[-t,0]}^x(t)|.\end{aligned}\tag{65}$$

Now, the objective is to bring (65) into the desired form (39). To this end, we start by exploiting the upper bounds of the candidate trajectories in (51), (52), and (53), yielding

$$\begin{aligned}|x(t) - \hat{x}(t)| &\leq \tilde{P}_0 |\hat{x}(0) - x(0)| \lambda^t + \sum_{\tau=1}^t \tilde{R}_0 |v(t - \tau)| \eta^\tau \\ &\quad + \sqrt{c_{\tilde{J}}(t, \bar{\varepsilon}_x^d, \bar{\varepsilon}_y^d)} 2r_2 \frac{\lambda - \lambda^{t+1}}{1 - \lambda} \sigma_{\max}^{\varepsilon_y} \\ &\quad + \sqrt{c_{\tilde{J}}(t, \bar{\varepsilon}_x^d, \bar{\varepsilon}_y^d)} c_\alpha (\bar{\varepsilon}_x^d + \bar{\varepsilon}_y^d) \alpha_{\max} \\ &\quad + \sqrt{c_{\tilde{J}}(t, \bar{\varepsilon}_x^d, \bar{\varepsilon}_y^d)} c_{\sigma^x} \sigma_{\max}^x.\end{aligned}\tag{66}$$

**Part II: Recursive Application of the Contraction Mapping** From here on, we consider  $t \geq L$ . Therefore,  $t$  must be replaced by  $L$  in the definition of the candidate solution (compare (43), (46), and (47)) and in the definition of  $c_{\tilde{J}}$  (see (41)). We reformulate (66) for all  $t \geq L$

$$\begin{aligned}|x(t) - \hat{x}(t)| &\leq \tilde{P}_0 |\hat{x}(t - L) - x(t - L)| \lambda^L \\ &\quad + \sum_{\tau=1}^L \tilde{R}_0 |v(t - \tau)| \eta^\tau \\ &\quad + \sqrt{c_{\tilde{J}, \max}} 2r_2 \frac{1 - \lambda^{L+1}}{1 - \lambda} \sigma_{\max}^{\varepsilon_y} \\ &\quad + \sqrt{c_{\tilde{J}, \max}} c_\alpha (\bar{\varepsilon}_x^d + \bar{\varepsilon}_y^d) \alpha_{\max} \\ &\quad + \sqrt{c_{\tilde{J}, \max}} c_{\sigma^x} \sigma_{\max}^x,\end{aligned}\tag{67}$$

where  $c_{\tilde{J}, \max} := \max\{c_{\tilde{J}}(L, \bar{\varepsilon}_x^d, \bar{\varepsilon}_y^d), c_{\tilde{J}}(0, \bar{\varepsilon}_x^d, \bar{\varepsilon}_y^d)\}$ . Inequality (67) establishes a contraction mapping from  $t - L$  up to time  $t$  for  $L$  large enough. The remaining steps regarding the terms  $x - \hat{x}$  and  $v$  are completely analogous to the previous section. Therefore, these steps are not explained in detail here. We focus on the additional terms that appear due to the considered noise in the offline phase. We choose  $L$  large enough so that  $\tilde{\mu} := \tilde{P}_0 \lambda^L \in (0, 1)$ . We apply the established contraction mapping recursively for  $t = TL + \tilde{t}$

$$\begin{aligned}|x(t) - \hat{x}(t)| &\leq \tilde{\mu}^T |x(t - TL) - \hat{x}(t - TL)| \\ &\quad + R_0 \sum_{k=0}^{T-1} \tilde{\mu}^k \sum_{\tau=1}^L |v(t - kL - \tau)| \lambda^\tau \\ &\quad + \sum_{k=0}^{T-1} \tilde{\mu}^k (c_4(\bar{\varepsilon}_x^d, \bar{\varepsilon}_y^d) \frac{\lambda - \lambda^{L+1}}{1 - \lambda} + c_5(\bar{\varepsilon}_x^d, \bar{\varepsilon}_y^d))\end{aligned}\tag{68}$$

for

$$c_4(\bar{\varepsilon}_x^d, \bar{\varepsilon}_y^d) := \sqrt{c_{\bar{J}, \max} 2r_2} \sigma_{\max}^{\varepsilon_y} \quad (69)$$

$$c_5(\bar{\varepsilon}_x^d, \bar{\varepsilon}_y^d) := \sqrt{c_{\bar{J}, \max} c_\alpha(\bar{\varepsilon}_x^d + \bar{\varepsilon}_y^d)} \alpha_{\max} + \sqrt{c_{\bar{J}, \max} c_{\sigma^x}} \sigma_{\max}^x. \quad (70)$$

We again replace the first term of inequality (68) with the expression obtained in (66) and get

$$\begin{aligned} |x(t) - \hat{x}(t)| &\leq \tilde{\mu}^T \left( \tilde{P}_0 |\hat{x}(0) - x(0)| \lambda^{\tilde{t}} + \sum_{\tau=1}^{\tilde{t}} \tilde{R}_0 |v(\tilde{t} - \tau)| \eta^\tau \right. \\ &\quad \left. + c_4(\bar{\varepsilon}_x^d, \bar{\varepsilon}_y^d) \frac{\lambda - \lambda^{\tilde{t}+1}}{1 - \lambda} + c_5(\bar{\varepsilon}_x^d, \bar{\varepsilon}_y^d) \right) \\ &\quad + R_0 \sum_{k=0}^{T-1} \tilde{\mu}^k \sum_{\tau=1}^L |v(t - kL - \tau)| \lambda^\tau \\ &\quad + \sum_{k=0}^{T-1} \tilde{\mu}^k (c_4(\bar{\varepsilon}_x^d, \bar{\varepsilon}_y^d) \frac{\lambda - \lambda^{L+1}}{1 - \lambda} + c_5(\bar{\varepsilon}_x^d, \bar{\varepsilon}_y^d)). \end{aligned}$$

The terms related to  $|\hat{x}(0) - x(0)|$  and  $v$  can be reformulated as in the previous section. We define  $\check{\lambda} := \tilde{\mu}^{1/L}$  and obtain

$$\begin{aligned} |x(t) - \hat{x}(t)| &\leq \tilde{P}_0 |\hat{x}(0) - x(0)| \check{\lambda}^t + \sum_{\tau=1}^t \tilde{R}_0 |v(t - \tau)| \check{\lambda}^\tau \\ &\quad + \tilde{\mu}^T (c_4(\bar{\varepsilon}_x^d, \bar{\varepsilon}_y^d) \frac{\lambda - \lambda^{\tilde{t}+1}}{1 - \lambda} + c_5(\bar{\varepsilon}_x^d, \bar{\varepsilon}_y^d)) \\ &\quad + \sum_{k=0}^{T-1} \tilde{\mu}^k (c_4(\bar{\varepsilon}_x^d, \bar{\varepsilon}_y^d) \frac{\lambda - \lambda^{L+1}}{1 - \lambda} + c_5(\bar{\varepsilon}_x^d, \bar{\varepsilon}_y^d)). \end{aligned}$$

Since  $\tilde{t} < L$ , this expression can be upper bounded by applying the geometric series

$$\begin{aligned} |x(t) - \hat{x}(t)| &\leq \tilde{P}_0 |\hat{x}(0) - x(0)| \check{\lambda}^t + \sum_{\tau=1}^t \tilde{R}_0 |v(t - \tau)| \check{\lambda}^\tau \\ &\quad + \frac{1 - \tilde{\mu}^{T+1}}{1 - \tilde{\mu}} (c_4(\bar{\varepsilon}_x^d, \bar{\varepsilon}_y^d) \frac{\lambda - \lambda^{L+1}}{1 - \lambda} + c_5(\bar{\varepsilon}_x^d, \bar{\varepsilon}_y^d)). \end{aligned}$$

Finally, we define

$$\gamma(\bar{\varepsilon}^d) := \frac{1}{1 - \tilde{\mu}} (c_4(\bar{\varepsilon}_x^d, \bar{\varepsilon}_y^d) \frac{\lambda - \lambda^{L+1}}{1 - \lambda} + c_5(\bar{\varepsilon}_x^d, \bar{\varepsilon}_y^d)), \quad (71)$$

such that  $\gamma \in \mathcal{K}$ . In particular, it holds that  $\gamma(0) = 0$ , since  $c_4(0, 0) = c_5(0, 0) = 0$ . This can be seen from (69) and (70). For  $\bar{\varepsilon}^d = 0$ , it follows that  $\sigma_{\max}^{\varepsilon_y} = 0$ , and  $\sigma_{\max}^x = 0$  (compare eqs. (53) and (52)), as well as  $\bar{\varepsilon}_x^d = \bar{\varepsilon}_y^d = 0$ . Note that

$$\frac{1 - \tilde{\mu}^{T+1}}{1 - \tilde{\mu}} (c_4(\bar{\varepsilon}_x^d, \bar{\varepsilon}_y^d) \frac{\lambda - \lambda^{L+1}}{1 - \lambda} + c_5(\bar{\varepsilon}_x^d, \bar{\varepsilon}_y^d)) \leq \gamma(\bar{\varepsilon}^d).$$

We obtain

$$\begin{aligned} |x(t) - \hat{x}(t)| &\leq \tilde{P}_0 |\hat{x}(0) - x(0)| \check{\lambda}^t + \sum_{\tau=1}^t \tilde{R}_0 |v(t - \tau)| \check{\lambda}^\tau \\ &\quad + \gamma(\bar{\varepsilon}^d), \end{aligned} \quad (72)$$

which proves that the data-driven MHE is pRES. ■

Note that if the upper bounds of the offline collected noise  $\bar{\varepsilon}_x^d$  and  $\bar{\varepsilon}_y^d$  tend to zero (i.e.,  $\bar{\varepsilon}^d$  tends to zero), we recover the case from the previous section since  $c_4(\bar{\varepsilon}_x^d, \bar{\varepsilon}_y^d)$  as well as  $c_5(\bar{\varepsilon}_x^d, \bar{\varepsilon}_y^d)$  and consequently  $\gamma(\bar{\varepsilon}^d)$  tend to zero, compare the reasoning below (71).

One inherent drawback of the applied proof technique is that the state estimation bound depends on the *a-priori* upper bound of the offline collected noise, which is more conservative than the actual noise levels  $\varepsilon_x^d$  and  $\varepsilon_y^d$ . This can be explained by the design of the cost function (38d) which considers the *a-priori* upper bounds of the offline collected noise. Hence, these bounds influence the final state estimation error bounds.



*Remark 5:* Throughout this work, we do not consider process noise, i.e., noise in the state dynamics of (5). Process noise is usually considered by an additional term  $w(t)$  added to the state equation (5a), resulting in

$$x(t+1) = Ax(t) + Bu(t) + w(t) \quad (73a)$$

$$\tilde{y}(t) = Cx(t) + Du(t) + v(t). \quad (73b)$$

We here discuss two options how process noise could be treated in the data-driven MHE scheme. First, one could assume that the process noise can be measured directly, as partly assumed in the context of data-driven MPC in [33]. In that case, the process noise could be treated as an additional input, where one would need to make sure that the concatenated control input  $u$  and the process noise input  $w$  fulfill the persistency of excitation assumption. The constraint (38c) would need to be augmented by the Hankel matrix containing the offline measured process noise trajectory and (regarding the online phase) by the measured process noise trajectory. However, the assumption that the process noise can be measured in practice is rarely fulfilled. Alternatively, if one does not consider that the process noise can be measured directly, one could incorporate the (unknown) process noise terms in the Hankel matrix composed of the offline measured state trajectory. Namely, if process noise is considered, the entries  $\tilde{x}^d(t)$  of the Hankel matrix  $H_{L+1}(\tilde{x}_{[0,N-1]}^d)$  on the left hand side of (38c) are given by

$$\begin{aligned} \tilde{x}^d(t) = & A^t \tilde{x}(0) + \sum_{i=0}^{t-1} A^{t-1-i} B u^d(i) \\ & + \sum_{i=0}^{t-1} A^{t-1-i} w^d(i) + \varepsilon_x^d(t). \end{aligned} \quad (74)$$

Consequently, the fitting error sequence  $\sigma^x$  must compensate (i) the measurement noise  $\varepsilon_x^d(t)$  corrupting the offline measured states and (ii) the cumulated process noise. The cumulated process noise would have to be bounded such that the term related to  $\sigma_{[-L,0]}^x(t)$  in the cost function remains bounded. Therefore, we would need to upper bound the maximal cumulated process noise at any time  $t$  by, e.g.,

$$\sum_{i=0}^{t-1} A^{t-1-i} w^d(i) \leq \sum_{i=0}^{t-1} |A^{t-1-i}|_{\infty} w_{\max}^d, \quad (75)$$

where  $w_{\max}^d$  is the maximal occurring process noise. This is possible if all eigenvalues of the matrix  $A$  are strictly inside the unit circle. Therefore, we would need to limit our analysis to stable systems (or pre-stabilized systems). In a related robust stability proof, one would need to treat the cumulated process noise as additional measurement noise and treat it similar to  $\varepsilon_x^d$ . However, this procedure would be very conservative, because all terms related to the (cumulated) process noise would need to be upper bounded by the maximum cumulated process noise (as it is the case in the dual problem of robust data-driven MPC, compare [34]). A quantitative analysis and/or the development of less conservative data-driven MHE schemes for the case of process noise is an interesting topic for future research.

*Remark 6:* The RGES proof in the previous Section III follows similar ideas than used in model-based MHE proof techniques. In contrast, the consideration of noise in the offline collected states and outputs in the current section renders the pRES proof substantially more complex and does not allow for a direct adaptation of model-based MHE stability proofs. In particular, noisy offline data are comparable to parametric uncertainty in model-based MHE (see, e.g., [35], [36]), since the Hankel matrices in (38) encode an implicit, uncertain “model” of the system.

## V. APPLICATION TO FOUR-TANK SYSTEM

In this section, we illustrate the performance of the novel robust data-driven MHE scheme by means of several numerical simulations. We consider exemplarily a four-tank system [37]. First, we focus on a linearized version of the four-tank system that has also been considered in [12]. Second, we consider the original nonlinear four-tank system. In both cases, we compare the performance of the data-driven MHE to the performance of a model-based MHE where the model is identified using the same (offline) input, output and state measurements that are used in the offline phase of the data-driven MHE formulation. In the context of controller design, some recent works compare the performance of direct data-driven control frameworks to indirect data-driven control frameworks, where in the latter the offline data are used to identify a model of the system, which is then used for model-based control, see [38], [39]. The main outcome of these works is that the indirect approach typically performs better if the offline data are only corrupted by measurement noise. In turn, direct data-based control can be superior if one faces a “bias error”, which can, e.g., result from identifying a linear model for a system which is, in fact, nonlinear, or when identifying a model of lower order than the real system dimension.

So far, these results are related to the control context. To the best of the authors’ knowledge, no investigations regarding the dual problem of estimation are available in the literature. Therefore, we here show a first comparison between direct data-driven MHE and indirect data-driven MHE by means of numerical experiments. In Subsection V-A we consider the linearized system with offline collected data that are subject to some additive measurement noise. In Subsection V-B, we consider exemplarily a bias error by identifying a four-dimensional linear model using data coming from a system that is, in fact, nonlinear.

### A. Linear System

The following linearized version of the open-loop stable four-tank system is considered

$$x(t+1) = \begin{bmatrix} 0.921 & 0 & 0.041 & 0 \\ 0 & 0.918 & 0 & 0.033 \\ 0 & 0 & 0.924 & 0 \\ 0 & 0 & 0 & 0.937 \end{bmatrix} x(t) + \begin{bmatrix} 0.017 & 0.001 \\ 0.001 & 0.023 \\ 0 & 0.061 \\ 0.072 & 0 \end{bmatrix} u(t) \quad (76a)$$

$$y(t) = \begin{bmatrix} 1 & 0 & 0 & 0 \\ 0 & 1 & 0 & 0 \end{bmatrix} x(t). \quad (76b)$$

In the following, we comment on the design of the data-driven MHE. We start by collecting  $N = 100$  input, output and state measurements of system (76), where the persistently exciting input is sampled from a uniform random distribution  $\mathcal{U}(0, 20)$ . The measurement noise regarding the offline collected outputs and states follows a truncated (at  $\pm 0.003$ ) normal distribution, i.e.,  $\varepsilon_x, \varepsilon_y \sim \mathcal{N}(\mu_{\mathcal{N}}, \sigma^2)$  with  $\mu_{\mathcal{N}} = 0$  and  $\sigma = 0.001$ . After the offline phase is completed, we construct the corresponding Hankel matrices using the measured inputs, states and outputs, and move to the online phase, where we apply a sinusoidal signal to both inputs.

Regarding the cost function, we choose  $\rho = 0.95$  (since  $\eta = 0.9337$  for system (76), where we determined the numerical value by means of the procedure outlined in Appendix A),  $c_\alpha = 2000$  and  $c_{\sigma^x} = 600$ . The upper bounds of the noise are chosen as  $\bar{\varepsilon}_x^d = \bar{\varepsilon}_y^d = 0.003$ . The weighting matrices are set to  $P = 500I_n$  and  $R_1 = 500I_p$  (and in a second run to  $R_2 = 2000I_p$ ) and the state constraint set  $\mathbb{X} = \{x \in \mathbb{R}^6 | x \geq 0\}$ , i.e., the water levels in the four tanks cannot be negative. The noise  $v$  corrupting the online output measurements follows a normal distribution with  $\mu_{\mathcal{N}} = 0$  and  $\sigma = 0.5$ . The horizon length is  $L = 7$ . The initial condition for system (76) in the online phase is  $x(0) = [7 \ 7 \ 7 \ 7]^\top$  and for the prior estimate  $\hat{x}(0) = [1 \ 2 \ 1 \ 2]^\top$ . The simulation results are illustrated in Figure 1, compare the estimates  $\hat{x}_{i,R_j}^{\text{DB}}$  for  $i \in \{1, \dots, 4\}$  and  $j \in \{1, 2\}$ . This figure illustrates that the robust data-driven MHE is pRES, as guaranteed by Theorem 3. Notice that, since  $x_1$  and  $x_2$  can be directly measured from the system (76), the corresponding estimations present only a small state estimation error.

As usual in MHE, the state estimates depend on the choice of the weighting matrix  $R$  (and, obviously, also on the choice of  $P$ ). It can be clearly seen in Figure 1 that a smaller value for  $R$  (here  $R_1$ ) induces a smoother estimated state trajectory. On the one hand, a higher value for  $R$  induces higher variations of the states estimates. On the other hand, the state estimates convergence (slightly) faster for a higher value of  $R$ . Loosely speaking, a high value for  $R$  implies that we prefer smaller values for  $\sigma^y$ , meaning that we trust our output measurements a lot. Since the output measurements are noisy, the corresponding state estimates are subject to fluctuations.

Regarding the design of the standard model-based MHE scheme, we first identify the matrices  $A$ ,  $B$ ,  $C$  (applying [19, Eq. (2.20)]) based on the same noisy data that we used to construct the Hankel matrices of the data-driven MHE scheme. Furthermore, we consider the same set-up, i.e., we chose the same weighing matrices  $P$ ,  $R_1$ ,  $R_2$ , the same discount factor  $\rho$ , the same horizon length  $L$ , the same noise realizations, and the same initial conditions  $x(0)$ ,  $\hat{x}(0)$ . According to the simulation results of Figure 1 (compare the estimates  $\hat{x}_{i,R_j}^{\text{MB}}$  for  $i \in \{1, \dots, 4\}$  and  $j \in \{1, 2\}$ ), the performance of the model-based MHE is very similar to the performance of the data-driven MHE.

### B. Nonlinear System

From here on, we consider the original nonlinear system, introduced in [37]

$$\dot{x}_1(t) = -\frac{a_1}{A_1} \sqrt{2gx_1(t)} + \frac{a_3}{A_1} \sqrt{2gx_3(t)} + \frac{\gamma_1}{A_1} u_1(t) \quad (77a)$$

$$\dot{x}_2(t) = -\frac{a_2}{A_2} \sqrt{2gx_2(t)} + \frac{a_4}{A_2} \sqrt{2gx_4(t)} + \frac{\gamma_2}{A_2} u_2(t) \quad (77b)$$

$$\dot{x}_3(t) = -\frac{a_3}{A_3} \sqrt{2gx_3(t)} + \frac{1-\gamma_2}{A_3} u_2(t) \quad (77c)$$

$$\dot{x}_4(t) = -\frac{a_4}{A_4} \sqrt{2gx_4(t)} + \frac{1-\gamma_1}{A_4} u_1(t). \quad (77d)$$

The numerical parameter values are given in [37]. Obviously, for this nonlinear case the derived robust stability guarantees do not hold anymore.

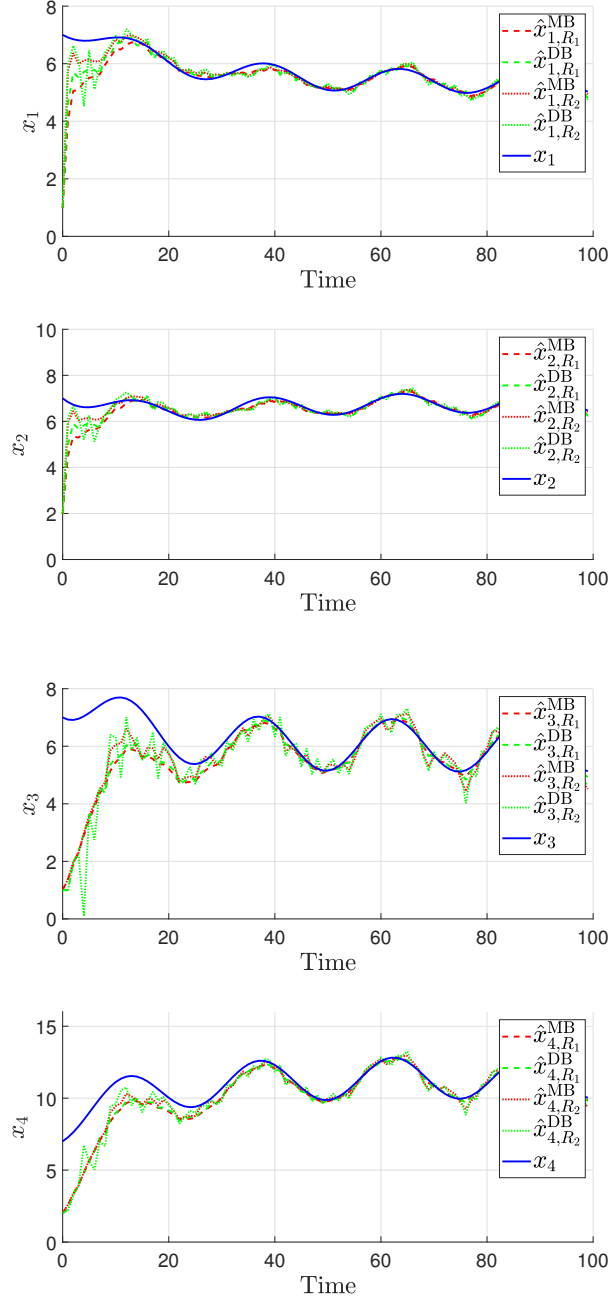

**Fig. 1:** The simulation results in this figure illustrate the performance of the robust data-driven MHE scheme (where the estimated states are denoted by  $\hat{x}^{DB}$ ) defined in (38) compared to a model-based MHE scheme (where the estimated states are denoted by  $\hat{x}^{MB}$ ) for the system (76). Two different values for the weighting matrix  $R$  are used.

In the offline phase, we apply a persistently exciting input to the system which is sampled from a uniform distribution  $\mathcal{U}(0, 20)$  and we collect  $N = 100$  samples from system (77). The measurement noise in the offline phase corrupting the output and state measurements follows a truncated (at  $\pm 0.003$ ) normal distribution with  $\mu_{\mathcal{N}} = 0$  and  $\sigma = 0.001$ . Once the data collection is completed, we switch to the online phase (in which we once again apply a sinusoidal signal).

The model-based and the data-driven MHE schemes are applied for the same parameters and the same initial condition for the true system dynamics and the prior estimate, i.e.,  $\rho, \mathbb{X}, P, R_1$  (and in a second run  $R_2$ ),  $L, x(0), \hat{x}(0)$  remain the same. Regarding the implementation of the data-driven MHE, the numerical values of  $c_\alpha, c_\sigma, \bar{\varepsilon}_x, \bar{\varepsilon}_y$  remain also unchanged. In order to implement a standard model-based MHE, we use the same noisy offline data collected from the nonlinear system (77) and identify a four-dimensional linear system such that we encounter a bias error.

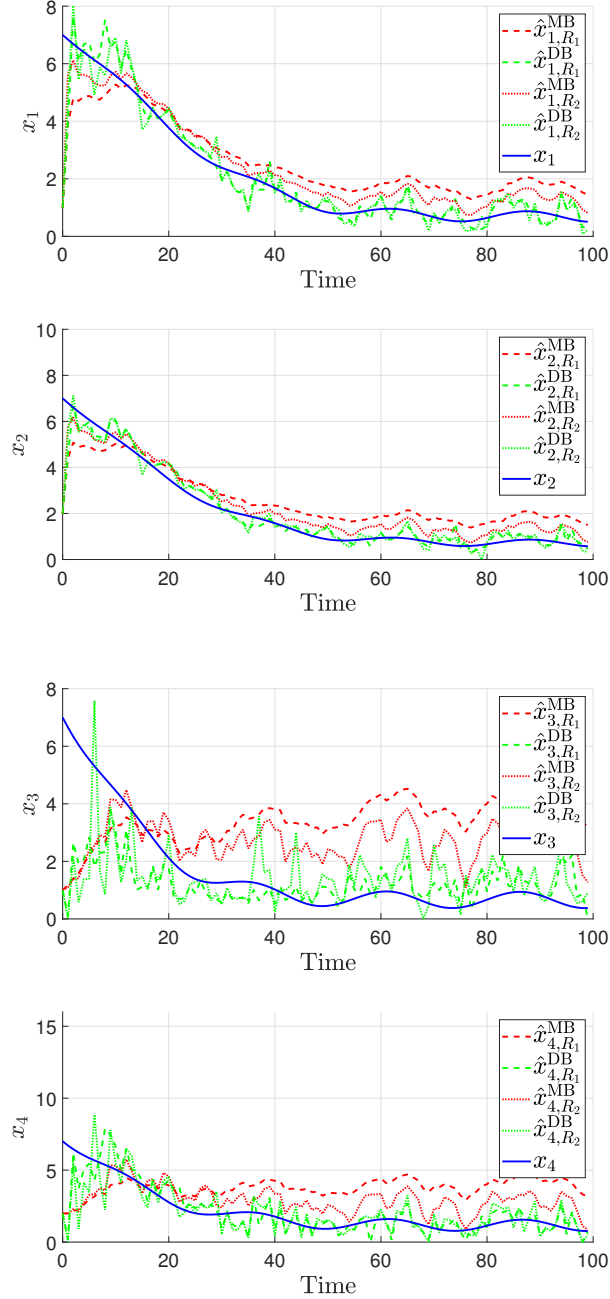

**Fig. 2:** The simulation results in this figure illustrate the performance of the robust data-driven MHE scheme defined in (38) compared to a model-based MHE scheme (where the model is identified using the same data) for the nonlinear system (77). Two different values for the weighting matrix  $R$  are used.

The simulation results are illustrated in Figure 2. In this figure, one can see that the performance of the direct data-driven MHE and indirect model-based MHE declines compared to the previous case (which is to be expected), where the considered system was linear.

However, the simulation results in Figure 2 suggest that the data-driven MHE performs better compared to the model-based MHE and can work well even in case that the underlying system is not linear. This observation is in line with the results from [38], [39], since we here deal with a bias error.

Based on these simulation results, one might ask for a conclusion regarding the question whether a direct data-driven MHE or an indirect data-driven MHE scheme is superior. On one side, we need to choose a value for the parameters  $c_{\sigma^x}$ ,  $c_\alpha$  and define the values of  $\bar{\varepsilon}_x^d$ ,  $\bar{\varepsilon}_y^d$  to implement the data-driven MHE scheme, which must not be done for the model-based MHE scheme simplifying its set-up. On the other side, the most important advantage of the data-driven MHE is that no

system identification is necessary, which enables a direct straight-forward application of the data-driven MHE. Furthermore, our simulation results suggest that direct data-driven MHE can be superior in case that an identified model would incur a bias error. A more comprehensive theoretical study of this issue (e.g., analogous to [38], [39]) is an interesting topic for future research.

## VI. CONCLUSION

In this paper, we showed RGES of a data-driven MHE scheme where the online measured outputs are corrupted by some persistent measurement noise. The obtained bounds are substantially improved compared to the preliminary conference version [20], by exploiting Jensen's inequality and an e-UOSS property considering discounting. In a further step, we relaxed the setting by allowing noisy offline collected states and outputs. To this end, we introduced a robust data-driven MHE scheme that considers regularization terms in the cost function so that the amplification of the offline collected noise is limited. We showed pRES for the novel robust data-driven MHE scheme. A numerical example illustrated the performance of the robust data-driven MHE scheme. Furthermore, we compared its performance to a standard model-based MHE scheme, where the same noisy offline data was used. Our simulation results revealed that the proposed direct data-driven MHE can be superior in case of a bias error.

Future work could focus on a variety of issues. First, our results are crucially based on the assumption that a potentially noisy state sequence is available from an offline phase. If one avoided this assumption, one could apply the robust MHE to a broader range of applications. Second, our theoretical guarantees are limited to linear systems, whereas MHE has been proven to be particularly powerful for nonlinear systems. Therefore, extending the here presented results to (specific classes of) nonlinear systems would be interesting. Third, this paper did not focus on a theoretical comparison between data-driven and model-based MHE schemes. In the dual problem of MPC, some first results concerning a theoretical comparison of data- and model-based MPC were obtained in [38], [39]. An interesting topic for future research would be a similar analysis in the context of MHE.

## APPENDIX

### A. Data-Driven Computation of e-UOSS Constants

Based on [29, Corollary 7], one can deduce that  $\eta$  can be chosen as  $\eta = |A_L|_{P_e}$ , where  $A_L$  corresponds to  $A_L = A + LC$  (with  $L$  such that  $A + LC$  is Schur stable) and  $P_e$  to the solution of [29, Eq. (28)]. Furthermore, the constants  $p_0$  and  $r_0$  can be chosen as  $p_0 = |P_e^{1/2}|/\sqrt{\lambda_{\min}(P_e)}$  and  $r_0 = |L|_{P_e}|P_e^{1/2}|$ . To obtain a data-driven expression of  $A_L$  (which then allows to compute  $P_e$  by means of [29, Eq. (28)]), we design a data-driven state feedback controller<sup>6</sup>  $L^\top$  for the dual system, as explained in [10], [17]. This controller leads to stable closed-loop dynamics, i.e.,  $A^\top + C^\top L^\top$  is Schur stable. Then, we take advantage of the duality between control and estimation. In fact, the stabilizing controller for the dual system is at the same time an observer for the original system with stable error dynamics. Furthermore, the closed-loop dynamics of the stabilized dual system (represented by  $A^\top + C^\top L^\top$  in the model-based system representation) correspond to  $A + LC$  of the original system, which allows to determine the required e-UOSS constants. Please note that this procedure is valid for noise-free (offline) data, as considered in Section III. Nevertheless, in simulations, we observe that this procedure still produces Schur stable matrices  $A_L$  (enabling a data-driven computation of the e-UOSS constants) as long as the noise level is small enough.

### B. State Estimation Error Bounds

As mentioned in Section III, we here want to show that  $c_J(t) > c_J(t+1) \forall t \in \mathbb{I}_{\geq 0}$  for  $\rho < \frac{p_0}{p_0+r_0}$ . To this end, we consider

$$p_0\rho^t + r_0\frac{\rho - \rho^{t+1}}{1 - \rho} > p_0\rho^{t+1} + r_0\frac{\rho - \rho^{t+2}}{1 - \rho}.$$

We multiply by  $1 - \rho$  and subtract  $r_0\rho$

$$p_0\rho^t(1 - \rho) - r_0\rho^{t+1} > p_0\rho^{t+1}(1 - \rho) - r_0\rho^{t+2}.$$

Dividing by  $\rho^t$  yields

$$p_0(1 - \rho) - r_0\rho > p_0\rho(1 - \rho) - r_0\rho^2.$$

This inequality can be reformulated as a quadratic expression in  $\rho$

$$\rho^2 - \rho\frac{2p_0 + r_0}{p_0 + r_0} + \frac{p_0}{p_0 + r_0} > 0, \quad (78)$$

which has its zeros at  $\rho_1 = 1$  and  $\rho_2 = \frac{p_0}{p_0+r_0}$ . Therefore, for any  $\rho < \frac{p_0}{p_0+r_0}$ , it holds that  $c_J(t) > c_J(t+1) \forall t \in \mathbb{I}_{\geq 0}$ .

<sup>6</sup>Note that the controller design requires data of the original system for which  $\text{rank}\left(\begin{bmatrix} H_1(x_{[1, N-1]}^d) \\ H_1(y_{[0, N-2]}^d) \end{bmatrix}\right) = n + p$  holds.

## REFERENCES

- [1] R. E. Kalman, "A new approach to linear filtering and prediction problems," *Transactions of the ASME—Journal of Basic Engineering*, vol. 82, pp. 35–45., 1960.
- [2] D. Luenberger, "An introduction to observers," *IEEE Transactions on Automatic Control*, vol. 16, no. 6, pp. 596–602, 1971.
- [3] J. B. Rawlings, D. Q. Mayne, and M. Diehl, *Model predictive control: theory, computation, and design*, 2nd ed. Nob Hill Publishing Madison, WI, 2020.
- [4] C. V. Rao, J. B. Rawlings, and J. H. Lee, "Constrained linear state estimation—a moving horizon approach," *Automatica*, vol. 37, no. 10, pp. 1619–1628, 2001.
- [5] A. Alessandri and M. Awawdeh, "Moving-horizon estimation for discrete-time linear systems with measurements subject to outliers," in *53rd IEEE Conference on Decision and Control*, 2014, pp. 2591–2596.
- [6] M. Gharbi and C. Ebenbauer, "Proximity moving horizon estimation for linear time-varying systems and a bayesian filtering view," in *2019 IEEE 58th Conference on Decision and Control (CDC)*. IEEE, 2019, pp. 3208–3213.
- [7] M. Farina, G. Ferrari-Trecate, and R. Scattolini, "Distributed moving horizon estimation for linear constrained systems," *IEEE Transactions on Automatic Control*, vol. 55, no. 11, pp. 2462–2475, 2010.
- [8] J. C. Willems, P. Rapisarda, I. Markovsky, and B. L. De Moor, "A note on persistency of excitation," *Systems & Control Letters*, vol. 54, no. 4, pp. 325–329, 2005.
- [9] I. Markovsky and P. Rapisarda, "Data-driven simulation and control," *International Journal of Control*, vol. 81, no. 12, pp. 1946–1959, 2008.
- [10] C. De Persis and P. Tesi, "Formulas for data-driven control: Stabilization, optimality, and robustness," *IEEE Transactions on Automatic Control*, vol. 65, no. 3, pp. 909–924, 2019.
- [11] J. Coulson, J. Lygeros, and F. Dörfler, "Data-enabled predictive control: In the shallows of the DeePC," in *2019 18th European Control Conference (ECC)*. IEEE, 2019, pp. 307–312.
- [12] J. Berberich, J. Köhler, M. A. Müller, and F. Allgöwer, "Data-driven model predictive control with stability and robustness guarantees," *IEEE Transactions on Automatic Control*, vol. 66, no. 4, pp. 1702–1717, 2020.
- [13] I. Markovsky and F. Dörfler, "Behavioral systems theory in data-driven analysis, signal processing, and control," *Annual Reviews in Control*, vol. 52, pp. 42–64, 2021.
- [14] V. G. Lopez and M. A. Müller, "On a continuous-time version of Willems' lemma," *accepted for CDC 2022, arXiv preprint arXiv:2203.03702*, 2022.
- [15] M. S. Turan and G. Ferrari-Trecate, "Data-driven unknown-input observers and state estimation," *IEEE Control Systems Letters*, vol. 6, pp. 1424–1429, 2022.
- [16] J. Shi, Y. Lian, and C. N. Jones, "Data-driven input reconstruction and experimental validation," *arXiv preprint arXiv:2203.02827*, 2022.
- [17] R. Adachi and Y. Wakasa, "Dual system representation and prediction method for data-driven estimation," in *2021 60th Annual Conference of the Society of Instrument and Control Engineers of Japan (SICE)*. IEEE, 2021, pp. 1245–1250.
- [18] A. Alanwar, A. Berndt, K. H. Johansson, and H. Sandberg, "Data-driven set-based estimation using matrix zonotopes with set containment guarantees," in *2022 European Control Conference (ECC)*. IEEE, 2022, pp. 875–881.
- [19] P. Van Overschee and B. De Moor, *Subspace identification for linear systems: Theory—Implementation—Applications*. Kluwer Academic Publishers, 1997.
- [20] T. M. Wolff, V. G. Lopez, and M. A. Müller, "Data-based moving horizon estimation for linear discrete-time systems," in *2022 European Control Conference (ECC)*. IEEE, 2022, pp. 1778–1783.
- [21] J. Berberich and F. Allgöwer, "A trajectory-based framework for data-driven system analysis and control," in *2020 European Control Conference (ECC)*. IEEE, 2020, pp. 1365–1370.
- [22] H. J. van Waarde, C. De Persis, M. K. Camlibel, and P. Tesi, "Willems' fundamental lemma for state-space systems and its extension to multiple datasets," *IEEE Control Systems Letters*, vol. 4, no. 3, pp. 602–607, 2020.
- [23] M. A. Müller, "Nonlinear moving horizon estimation in the presence of bounded disturbances," *Automatica*, vol. 79, pp. 306–314, 2017.
- [24] D. A. Allan and J. B. Rawlings, "Moving horizon estimation," in *Handbook of Model Predictive Control*, S. V. Raković and W. S. Levine, Eds. Cham: Springer International Publishing, 2019, pp. 99–124.
- [25] S. Knüfer and M. A. Müller, "Robust global exponential stability for moving horizon estimation," in *2018 IEEE Conference on Decision and Control (CDC)*, 2018, pp. 3477–3482.
- [26] S. Knüfer and M. A. Müller, "Nonlinear full information and moving horizon estimation: Robust global asymptotic stability," *arXiv preprint arXiv:2105.02764*, 2021.
- [27] D. A. Allan and J. B. Rawlings, "Robust stability of full information estimation," *SIAM Journal on Control and Optimization*, vol. 59, no. 5, pp. 3472–3497, 2021.
- [28] J. D. Schiller and M. A. Müller, "Suboptimal nonlinear moving horizon estimation," *accepted for IEEE Transactions on Automatic Control*, 2022.
- [29] S. Knüfer and M. A. Müller, "Time-discounted incremental input/output-to-state stability," in *2020 59th IEEE Conference on Decision and Control (CDC)*. IEEE, 2020, pp. 5394–5400.
- [30] J. L. W. V. Jensen, "Sur les fonctions convexes et les inégalités entre les valeurs moyennes," *Acta mathematica*, vol. 30, no. 1, pp. 175–193, 1906.
- [31] J. D. Schiller, S. Muntwiler, J. Köhler, M. N. Zeilinger, and M. A. Müller, "A Lyapunov function for robust stability of moving horizon estimation," *arXiv preprint arXiv:2202.12744*, 2022.
- [32] J. Coulson, J. Lygeros, and F. Dörfler, "Regularized and distributionally robust data-enabled predictive control," in *2019 IEEE 58th Conference on Decision and Control (CDC)*. IEEE, 2019, pp. 2696–2701.
- [33] G. Pan, R. Ou, and T. Faulwasser, "On a stochastic fundamental lemma and its use for data-driven MPC," *arXiv preprint arXiv:2111.13636*, 2021.
- [34] C. Klöppelt, J. Berberich, F. Allgöwer, and M. A. Müller, "A novel constraint tightening approach for robust data-driven predictive control," *arXiv preprint arXiv:2203.07055*, 2022.
- [35] A. Alessandri, M. Baglietto, and G. Battistelli, "Robust receding-horizon state estimation for uncertain discrete-time linear systems," *Systems & Control Letters*, vol. 54, no. 7, pp. 627–643, 2005.
- [36] —, "Min-max moving-horizon estimation for uncertain discrete-time linear systems," *SIAM Journal on Control and Optimization*, vol. 50, no. 3, pp. 1439–1465, 2012.
- [37] T. Raff, S. Huber, Z. K. Nagy, and F. Allgöwer, "Nonlinear model predictive control of a four tank system: An experimental stability study," in *2006 IEEE International Conference on Control Applications*. IEEE, 2006, pp. 237–242.
- [38] F. Dörfler, J. Coulson, and I. Markovsky, "Bridging direct & indirect data-driven control formulations via regularizations and relaxations," *IEEE Transactions on Automatic Control*, 2022.
- [39] V. Krishnan and F. Pasqualetti, "On direct vs indirect data-driven predictive control," in *2021 60th IEEE Conference on Decision and Control (CDC)*, 2021, pp. 736–741.



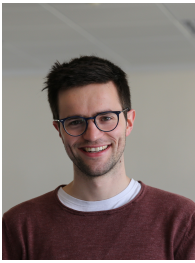

**Tobias M. Wolff** received a M.Sc. degree in Electrical Engineering from the Karlsruhe Institute of Technology and from the Grenoble Institute of Technology, both in 2021. He is currently a PhD student at the Institute of Automatic Control, Leibniz University Hannover, Germany. His main research interests are data- and learning-based estimation and biomedical applications.

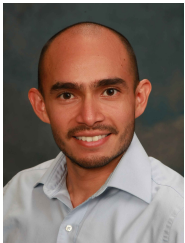

**Victor G. Lopez** received his B.Sc. degree in Communications and Electronics Engineering from the Universidad Autonoma de Campeche, in Campeche, Mexico, in 2010, the M.Sc. degree in Electrical Engineering from the Research and Advanced Studies Center (Cinvestav), in Guadalajara, Mexico, in 2013, and his Ph.D. degree in Electrical Engineering from the University of Texas at Arlington, Texas, USA, in 2019. In 2015 Victor was a Lecturer at the Western Technological Institute of Superior Studies (ITESO) in Guadalajara, Mexico. From August 2019 to June 2020, he was a postdoctoral researcher at the University of Texas at Arlington Research Institute and an Adjunct Professor in the Electrical Engineering department at UTA. Victor is currently a postdoctoral researcher at the Institute of Automatic Control, Leibniz University Hannover, Germany. His research interest include cyber-physical systems, reinforcement learning, game theory, distributed control and robust control.

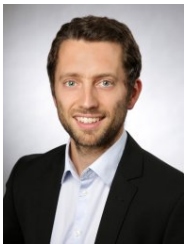

**Matthias A. Müller** received a Diploma degree in Engineering Cybernetics from the University of Stuttgart, Germany, and an M.S. in Electrical and Computer Engineering from the University of Illinois at Urbana-Champaign, US, both in 2009. In 2014, he obtained a Ph.D. in Mechanical Engineering, also from the University of Stuttgart, Germany, for which he received the 2015 European Ph.D. award on control for complex and heterogeneous systems. Since 2019, he is director of the Institute of Automatic Control and full professor at the Leibniz University Hannover, Germany. He obtained an ERC Starting Grant in 2020 and is recipient of the inaugural Brockett-Willems Outstanding Paper Award for the best paper published in Systems & Control Letters in the period 2014-2018. His research interests include nonlinear control and estimation, model predictive control, and data-/learning-based control, with application in different fields including biomedical engineering.
